# Supplementary material for: Multimodal Image Denoising based on Coupled Dictionary Learning
Source: arXiv:1806.10678 source file (2018-06-26)
Supplement: Supplementary file 1 [file Appendices_V2.tex]

\mypar{Appendix: More Experiments}
% Introduction to T1 and T2 characteristics.

In this appendix, we provide more experiment results for demonstration of our algorithm.

%\section{Experiments}
%\label{sec:Experiments}
%\vspace{-0.2cm}

%
%% Training images
\begin{figure*}[bhtp]
	\centering
	% ------------------------------------------- 
	%	\begin{minipage}[b]{0.06\linewidth}
	%		\centering
	%		{\footnotesize Infrared} \hfill % \vfill
	%		{\footnotesize RGB}
	%	\end{minipage} 
	\begin{minipage}[b]{0.1\linewidth}
		\centering
		\includegraphics[width = 1.8cm, height = 1.8cm]{./Figures/Dataset/Train_RGB_NIR/train-0.png}
		\includegraphics[width = 1.8cm, height = 1.8cm]{./Figures/Dataset/Train_RGB_NIR/train-1.png}
	\end{minipage} 
	\begin{minipage}[b]{0.1\linewidth}
		\centering
		\includegraphics[width = 1.8cm, height = 1.8cm]{./Figures/Dataset/Train_RGB_NIR/train-2.png}
		\includegraphics[width = 1.8cm, height = 1.8cm]{./Figures/Dataset/Train_RGB_NIR/train-3.png}
	\end{minipage} 
	\begin{minipage}[b]{0.1\linewidth}
		\centering
		\includegraphics[width = 1.8cm, height = 1.8cm]{./Figures/Dataset/Train_RGB_NIR/train-4.png}
		\includegraphics[width = 1.8cm, height = 1.8cm]{./Figures/Dataset/Train_RGB_NIR/train-5.png}
	\end{minipage} 
	\begin{minipage}[b]{0.1\linewidth}
		\centering
		\includegraphics[width = 1.8cm, height = 1.8cm]{./Figures/Dataset/Train_RGB_NIR/train-6.png}
		\includegraphics[width = 1.8cm, height = 1.8cm]{./Figures/Dataset/Train_RGB_NIR/train-7.png}
	\end{minipage} 
	\begin{minipage}[b]{0.1\linewidth}
		\centering
		\includegraphics[width = 1.8cm, height = 1.8cm]{./Figures/Dataset/Train_RGB_NIR/train-8.png}
		\includegraphics[width = 1.8cm, height = 1.8cm]{./Figures/Dataset/Train_RGB_NIR/train-9.png}
	\end{minipage} 
	\begin{minipage}[b]{0.1\linewidth}
		\centering
		\includegraphics[width = 1.8cm, height = 1.8cm]{./Figures/Dataset/Train_RGB_NIR/train-10.png}
		\includegraphics[width = 1.8cm, height = 1.8cm]{./Figures/Dataset/Train_RGB_NIR/train-11.png}
	\end{minipage} 
	\begin{minipage}[b]{0.1\linewidth}
		\centering
		\includegraphics[width = 1.8cm, height = 1.8cm]{./Figures/Dataset/Train_RGB_NIR/train-12.png}
		\includegraphics[width = 1.8cm, height = 1.8cm]{./Figures/Dataset/Train_RGB_NIR/train-13.png}
	\end{minipage} 
	\begin{minipage}[b]{0.1\linewidth}
		\centering
		\includegraphics[width = 1.8cm, height = 1.8cm]{./Figures/Dataset/Train_RGB_NIR/train-14.png}
		\includegraphics[width = 1.8cm, height = 1.8cm]{./Figures/Dataset/Train_RGB_NIR/train-15.png}
	\end{minipage} 
	\begin{minipage}[b]{0.1\linewidth}
		\centering
		\includegraphics[width = 1.8cm, height = 1.8cm]{./Figures/Dataset/Train_RGB_NIR/train-16.png}
		\includegraphics[width = 1.8cm, height = 1.8cm]{./Figures/Dataset/Train_RGB_NIR/train-17.png}
	\end{minipage} 
	\\
	% ------------------------------------------- 
	% ------------------------------------------- 
	%	\begin{minipage}[b]{0.06\linewidth}
	%		\centering	{\phantom{{\footnotesize Methods}}} 
	%	\end{minipage}
	%	\begin{minipage}[b]{0.15\linewidth}
	%		\centering	{\footnotesize $\sigma=4$}
	%	\end{minipage} 
	% -------------------------------------------	
	\caption{Some training infrared/RGB image pairs. The first row represents the infrared images and the second row represents the corresponding RGB images.}
	\label{Fig:TrainIms}
\end{figure*}
%
%
%% Testing images
\begin{figure*}[bhtp]
	\centering
	% ------------------------------------------- 
	%	\begin{minipage}[b]{0.06\linewidth}
	%		\centering
	%		{\footnotesize Infrared} \hfill % \vfill
	%		{\footnotesize RGB}
	%	\end{minipage} 
	\begin{minipage}[b]{0.11\linewidth}
		\centering
		\includegraphics[width = 2cm, height = 2cm]{./Figures/Dataset/Test_RGB_NIR/result-0.png}
		\includegraphics[width = 2cm, height = 2cm]{./Figures/Dataset/Test_RGB_NIR/result-1.png}
	\end{minipage} 
	\begin{minipage}[b]{0.11\linewidth}
		\centering
		\includegraphics[width = 2cm, height = 2cm]{./Figures/Dataset/Test_RGB_NIR/result-2.png}
		\includegraphics[width = 2cm, height = 2cm]{./Figures/Dataset/Test_RGB_NIR/result-3.png}
	\end{minipage} 
	\begin{minipage}[b]{0.11\linewidth}
		\centering
		\includegraphics[width = 2cm, height = 2cm]{./Figures/Dataset/Test_RGB_NIR/result-4.png}
		\includegraphics[width = 2cm, height = 2cm]{./Figures/Dataset/Test_RGB_NIR/result-5.png}
	\end{minipage} 
	\begin{minipage}[b]{0.11\linewidth}
		\centering
		\includegraphics[width = 2cm, height = 2cm]{./Figures/Dataset/Test_RGB_NIR/result-6.png}
		\includegraphics[width = 2cm, height = 2cm]{./Figures/Dataset/Test_RGB_NIR/result-7.png}
	\end{minipage} 
	\begin{minipage}[b]{0.11\linewidth}
		\centering
		\includegraphics[width = 2cm, height = 2cm]{./Figures/Dataset/Test_RGB_NIR/result-8.png}
		\includegraphics[width = 2cm, height = 2cm]{./Figures/Dataset/Test_RGB_NIR/result-9.png}
	\end{minipage} 
	\begin{minipage}[b]{0.11\linewidth}
		\centering
		\includegraphics[width = 2cm, height = 2cm]{./Figures/Dataset/Test_RGB_NIR/result-10.png}
		\includegraphics[width = 2cm, height = 2cm]{./Figures/Dataset/Test_RGB_NIR/result-11.png}
	\end{minipage} 
	\begin{minipage}[b]{0.11\linewidth}
		\centering
		\includegraphics[width = 2cm, height = 2cm]{./Figures/Dataset/Test_RGB_NIR/result-12.png}
		\includegraphics[width = 2cm, height = 2cm]{./Figures/Dataset/Test_RGB_NIR/result-13.png}
	\end{minipage} 
	\begin{minipage}[b]{0.11\linewidth}
		\centering
		\includegraphics[width = 2cm, height = 2cm]{./Figures/Dataset/Test_RGB_NIR/result-14.png}
		\includegraphics[width = 2cm, height = 2cm]{./Figures/Dataset/Test_RGB_NIR/result-15.png}
	\end{minipage} 
	\\
	% ------------------------------------------- 
	\begin{minipage}[b]{0.11\linewidth}
		\centering {\footnotesize urban 0004}
	\end{minipage} 
	\begin{minipage}[b]{0.11\linewidth}
		\centering {\footnotesize urban 0006}
	\end{minipage} 
	\begin{minipage}[b]{0.11\linewidth}
		\centering {\footnotesize urban 0017}
	\end{minipage} 
	\begin{minipage}[b]{0.11\linewidth}
		\centering {\footnotesize urban 0018}
	\end{minipage} 
	\begin{minipage}[b]{0.11\linewidth}
		\centering {\footnotesize urban 0020}
	\end{minipage} 
	\begin{minipage}[b]{0.11\linewidth}
		\centering {\footnotesize urban 0026}
	\end{minipage} 
	\begin{minipage}[b]{0.11\linewidth}
		\centering {\footnotesize urban 0030}
	\end{minipage} 
	\begin{minipage}[b]{0.11\linewidth}
		\centering {\footnotesize urban 0050}
	\end{minipage} 
	% ------------------------------------------- 
	\caption{Some testing infrared/RGB image pairs. The first row represents the infrared images and the second row represents the corresponding RGB images.}
	\label{Fig:TestIms}
\end{figure*}

\begin{figure*}[th]
	\begin{multicols}{2}  
		\centering
		% ------------------------------------------- 
		% Noisy images
		\begin{minipage}[b]{0.1\linewidth}
			\centering
			{\footnotesize Input}  
		\end{minipage} 
		\begin{minipage}[b]{0.28\linewidth}
			\centering
			\includegraphics[width = 2.5cm, height = 2.5cm]{./Figures/GF/ImgNo1_Noise8_X_low.eps}
		\end{minipage} 
		\begin{minipage}[b]{0.28\linewidth}
			\centering
			\includegraphics[width = 2.5cm, height = 2.5cm]{./Figures/GF/ImgNo1_Noise16_X_low.eps}
		\end{minipage} 
		\begin{minipage}[b]{0.28\linewidth}
			\centering
			\includegraphics[width = 2.5cm, height = 2.5cm]{./Figures/GF/ImgNo1_Noise24_X_low.eps}
		\end{minipage} 
		\\
		% ------------------------------------------- 
		% JBF
		\begin{minipage}[b]{0.1\linewidth}
			\centering
			{\footnotesize JBF~\cite{kopf2007joint}} % 
		\end{minipage} 
		\begin{minipage}[b]{0.28\linewidth}
			\centering
			\includegraphics[width = 2.5cm, height = 2.5cm]{./Figures/JBF/ImgNo1_Noise8_X_JBF.eps}
		\end{minipage}  
		\begin{minipage}[b]{0.28\linewidth}
			\centering
			\includegraphics[width = 2.5cm, height = 2.5cm]{./Figures/JBF/ImgNo1_Noise16_X_JBF.eps}
		\end{minipage} 
		\begin{minipage}[b]{0.28\linewidth}
			\centering
			\includegraphics[width = 2.5cm, height = 2.5cm]{./Figures/JBF/ImgNo1_Noise24_X_JBF.eps}
		\end{minipage} 
		\\
		% ------------------------------------------- 
		% JBF
		\begin{minipage}[b]{0.1\linewidth}
			\centering
			{\footnotesize ErrMap JBF~\cite{kopf2007joint}} % 
		\end{minipage} 
		\begin{minipage}[b]{0.28\linewidth}
			\centering
			\includegraphics[width = 2.5cm, height = 2.5cm]{./Figures/JBF/ImgNo1_Noise8_X_resid_JBF.eps}
		\end{minipage} 
		\begin{minipage}[b]{0.28\linewidth}
			\centering
			\includegraphics[width = 2.5cm, height = 2.5cm]{./Figures/JBF/ImgNo1_Noise16_X_resid_JBF.eps}
		\end{minipage} 
		\begin{minipage}[b]{0.28\linewidth}
			\centering
			\includegraphics[width = 2.5cm, height = 2.5cm]{./Figures/JBF/ImgNo1_Noise24_X_resid_JBF.eps}
		\end{minipage} 
		\\
		% ------------------------------------------- 
		% GF
		\begin{minipage}[b]{0.1\linewidth}
			\centering
			{\footnotesize GF~\cite{he2013guided}}  
		\end{minipage}  
		\begin{minipage}[b]{0.28\linewidth}
			\centering
			\includegraphics[width = 2.5cm, height = 2.5cm]{./Figures/GF/ImgNo1_Noise8_X_GF.eps}
		\end{minipage} 
		\begin{minipage}[b]{0.28\linewidth}
			\centering
			\includegraphics[width = 2.5cm, height = 2.5cm]{./Figures/GF/ImgNo1_Noise16_X_GF.eps}
		\end{minipage} 
		\begin{minipage}[b]{0.28\linewidth}
			\centering
			\includegraphics[width = 2.5cm, height = 2.5cm]{./Figures/GF/ImgNo1_Noise24_X_GF.eps}
		\end{minipage} 
		\\
		% ------------------------------------------- 
		% GF
		\begin{minipage}[b]{0.1\linewidth}
			\centering
			{\footnotesize ErrMap GF~\cite{he2013guided}}  
		\end{minipage} 
		\begin{minipage}[b]{0.28\linewidth}
			\centering
			\includegraphics[width = 2.5cm, height = 2.5cm]{./Figures/GF/ImgNo1_Noise8_X_resid_GF.eps}
		\end{minipage} 
		\begin{minipage}[b]{0.28\linewidth}
			\centering
			\includegraphics[width = 2.5cm, height = 2.5cm]{./Figures/GF/ImgNo1_Noise16_X_resid_GF.eps}
		\end{minipage} 
		\begin{minipage}[b]{0.28\linewidth}
			\centering
			\includegraphics[width = 2.5cm, height = 2.5cm]{./Figures/GF/ImgNo1_Noise24_X_resid_GF.eps}
		\end{minipage} 
		\\
		% -------------------------------------------
		% SDF
		\begin{minipage}[b]{0.1\linewidth}
			\centering
			{\footnotesize SDF~\cite{ham2017robust}} %  
		\end{minipage} 
		\begin{minipage}[b]{0.28\linewidth}
			\centering
			\includegraphics[width = 2.5cm, height = 2.5cm]{./Figures/SDF/ImgNo1_Noise8_X_SDF.eps}
		\end{minipage} 
		\begin{minipage}[b]{0.28\linewidth}
			\centering
			\includegraphics[width = 2.5cm, height = 2.5cm]{./Figures/SDF/ImgNo1_Noise16_X_SDF.eps}
		\end{minipage}  
		\begin{minipage}[b]{0.28\linewidth}
			\centering
			\includegraphics[width = 2.5cm, height = 2.5cm]{./Figures/SDF/ImgNo1_Noise24_X_SDF.eps}
		\end{minipage} 
		\\
		% -------------------------------------------
		% SDF
		\begin{minipage}[b]{0.1\linewidth}
			\centering
			{\footnotesize ErrMap SDF~\cite{ham2017robust}} % 
		\end{minipage}  
		\begin{minipage}[b]{0.28\linewidth}
			\centering
			\includegraphics[width = 2.5cm, height = 2.5cm]{./Figures/SDF/ImgNo1_Noise8_X_resid_SDF.eps}
		\end{minipage} 
		\begin{minipage}[b]{0.28\linewidth}
			\centering
			\includegraphics[width = 2.5cm, height = 2.5cm]{./Figures/SDF/ImgNo1_Noise16_X_resid_SDF.eps}
		\end{minipage} 
		\begin{minipage}[b]{0.28\linewidth}
			\centering
			\includegraphics[width = 2.5cm, height = 2.5cm]{./Figures/SDF/ImgNo1_Noise24_X_resid_SDF.eps}
		\end{minipage} 
		\\
		% ------------------------------------------- 
		\begin{minipage}[b]{0.1\linewidth}
			\centering	% {\phantom{{\footnotesize XXX}}} 
		\end{minipage}
		\begin{minipage}[b]{0.28\linewidth}
			\centering	{\footnotesize $\sigma=8$}
		\end{minipage} 
		\begin{minipage}[b]{0.28\linewidth}
			\centering	{\footnotesize $\sigma=16$} 
		\end{minipage} 
		\begin{minipage}[b]{0.28\linewidth}
			\centering	{\footnotesize $\sigma=24$} 
		\end{minipage}
		\\
		%---------------------------------------------------
		% true images
		\begin{minipage}[b]{0.1\linewidth}
			\centering
			{\footnotesize Truth}  
		\end{minipage} 
		\begin{minipage}[b]{0.28\linewidth}
			\centering
			\includegraphics[width = 2.5cm, height = 2.5cm]{./Figures/GF/ImgNo1_Noise8_X_true.eps}
		\end{minipage} 
		\begin{minipage}[b]{0.28\linewidth}
			\centering
			\includegraphics[width = 2.5cm, height = 2.5cm]{./Figures/GF/ImgNo1_Noise16_X_true.eps}
		\end{minipage} 
		\begin{minipage}[b]{0.28\linewidth}
			\centering
			\includegraphics[width = 2.5cm, height = 2.5cm]{./Figures/GF/ImgNo1_Noise24_X_true.eps}
		\end{minipage} 
		\\
		% -------------------------------------------
		% JFSM
		\begin{minipage}[b]{0.1\linewidth}
			\centering
			{\footnotesize JFSM\cite{shen2015multispectral}}  
		\end{minipage}  
		\begin{minipage}[b]{0.28\linewidth}
			\centering
			\includegraphics[width = 2.5cm, height = 2.5cm]{./Figures/JFSM/ImgNo1_Noise8_X_JFSM.eps}
		\end{minipage}  
		\begin{minipage}[b]{0.28\linewidth}
			\centering
			\includegraphics[width = 2.5cm, height = 2.5cm]{./Figures/JFSM/ImgNo1_Noise16_X_JFSM.eps}
		\end{minipage} 
		\begin{minipage}[b]{0.28\linewidth}
			\centering
			\includegraphics[width = 2.5cm, height = 2.5cm]{./Figures/JFSM/ImgNo1_Noise24_X_JFSM.eps}
		\end{minipage} 
		\\
		% -------------------------------------------	
		% JFSM
		\begin{minipage}[b]{0.1\linewidth}
			\centering
			{\footnotesize ErrMap JFSM\cite{shen2015multispectral}}  
		\end{minipage} 
		\begin{minipage}[b]{0.28\linewidth}
			\centering
			\includegraphics[width = 2.5cm, height = 2.5cm]{./Figures/JFSM/ImgNo1_Noise8_X_resid_JFSM.eps}
		\end{minipage} 
		\begin{minipage}[b]{0.28\linewidth}
			\centering
			\includegraphics[width = 2.5cm, height = 2.5cm]{./Figures/JFSM/ImgNo1_Noise16_X_resid_JFSM.eps}
		\end{minipage} 
		\begin{minipage}[b]{0.28\linewidth}
			\centering
			\includegraphics[width = 2.5cm, height = 2.5cm]{./Figures/JFSM/ImgNo1_Noise24_X_resid_JFSM.eps}
		\end{minipage} 
		\\
		% -------------------------------------------
		% DJF
		\begin{minipage}[b]{0.1\linewidth}
			\centering
			{\footnotesize DJF~\cite{li2016deep}} %  
		\end{minipage} 
		\begin{minipage}[b]{0.28\linewidth}
			\centering
			\includegraphics[width = 2.5cm, height = 2.5cm]{./Figures/DJF/ImgNo1_Noise8_X_DJF.eps}
		\end{minipage} 
		\begin{minipage}[b]{0.28\linewidth}
			\centering
			\includegraphics[width = 2.5cm, height = 2.5cm]{./Figures/DJF/ImgNo1_Noise16_X_DJF.eps}
		\end{minipage} 
		\begin{minipage}[b]{0.28\linewidth}
			\centering
			\includegraphics[width = 2.5cm, height = 2.5cm]{./Figures/DJF/ImgNo1_Noise24_X_DJF.eps}
		\end{minipage} 
		\\
		% -------------------------------------------
		% DJF
		\begin{minipage}[b]{0.1\linewidth}
			\centering
			{\footnotesize ErrMap DJF~\cite{li2016deep}} %  
		\end{minipage}  
		\begin{minipage}[b]{0.28\linewidth}
			\centering
			\includegraphics[width = 2.5cm, height = 2.5cm]{./Figures/DJF/ImgNo1_Noise8_X_resid_DJF.eps}
		\end{minipage} 
		\begin{minipage}[b]{0.28\linewidth}
			\centering
			\includegraphics[width = 2.5cm, height = 2.5cm]{./Figures/DJF/ImgNo1_Noise16_X_resid_DJF.eps}
		\end{minipage} 
		\begin{minipage}[b]{0.28\linewidth}
			\centering
			\includegraphics[width = 2.5cm, height = 2.5cm]{./Figures/DJF/ImgNo1_Noise24_X_resid_DJF.eps}
		\end{minipage} 
		\\
		% -------------------------------------------
		%	% CDN with standard sparsity
		%	\begin{minipage}[b]{0.1\linewidth}
		%		\centering
		%		{\footnotesize Ours} %  
		%	\end{minipage} 
		%	\begin{minipage}[b]{0.28\linewidth}
		%		\centering
		%		\includegraphics[width = 2.5cm, height = 2.5cm]{./Figures/CDN/ImgNo1_Noise4_X_CDN.eps}
		%	\end{minipage} 
		%	\begin{minipage}[b]{0.28\linewidth}
		%		\centering
		%		\includegraphics[width = 2.5cm, height = 2.5cm]{./Figures/CDN/ImgNo1_Noise12_X_CDN.eps}
		%	\end{minipage} 
		%	\begin{minipage}[b]{0.28\linewidth}
		%		\centering
		%		\includegraphics[width = 2.5cm, height = 2.5cm]{./Figures/CDN/ImgNo1_Noise20_X_CDN.eps}
		%	\end{minipage} 
		%	\\
		% -------------------------------------------
		%	% CDN with standard sparsity
		%	\begin{minipage}[b]{0.1\linewidth}
		%		\centering
		%		{\footnotesize ErrMap Ours} %  
		%	\end{minipage} 
		%	\begin{minipage}[b]{0.28\linewidth}
		%		\centering
		%		\includegraphics[width = 2.5cm, height = 2.5cm]{./Figures/CDN/ImgNo1_Noise8_X_resid_CDN.eps}
		%	\end{minipage} 
		%	\begin{minipage}[b]{0.28\linewidth}
		%		\centering
		%		\includegraphics[width = 2.5cm, height = 2.5cm]{./Figures/CDN/ImgNo1_Noise16_X_resid_CDN.eps}
		%	\end{minipage} 
		%	\begin{minipage}[b]{0.28\linewidth}
		%		\centering
		%		\includegraphics[width = 2.5cm, height = 2.5cm]{./Figures/CDN/ImgNo1_Noise24_X_resid_CDN.eps}
		%	\end{minipage} 
		%	\\
		% -------------------------------------------
		% CDN with group sparsity
		\begin{minipage}[b]{0.1\linewidth}
			\centering
			{\footnotesize Ours+}  
		\end{minipage} 
		\begin{minipage}[b]{0.28\linewidth}
			\centering
			\includegraphics[width = 2.5cm, height = 2.5cm]{./Figures/CDN_GrpSp/ImgNo1_Noise8_X_CDN.eps}
		\end{minipage} 
		\begin{minipage}[b]{0.28\linewidth}
			\centering
			\includegraphics[width = 2.5cm, height = 2.5cm]{./Figures/CDN_GrpSp/ImgNo1_Noise16_X_CDN.eps}
		\end{minipage} 
		\begin{minipage}[b]{0.28\linewidth}
			\centering
			\includegraphics[width = 2.5cm, height = 2.5cm]{./Figures/CDN_GrpSp/ImgNo1_Noise24_X_CDN.eps}
		\end{minipage} 
		\\
		% -------------------------------------------
		% CDN with group sparsity
		\begin{minipage}[b]{0.1\linewidth}
			\centering
			{\footnotesize ErrMap Ours+}  
		\end{minipage} 
		\begin{minipage}[b]{0.28\linewidth}
			\centering
			\includegraphics[width = 2.5cm, height = 2.5cm]{./Figures/CDN_GrpSp/ImgNo1_Noise8_X_resid_CDN.eps}
		\end{minipage} 
		\begin{minipage}[b]{0.28\linewidth}
			\centering
			\includegraphics[width = 2.5cm, height = 2.5cm]{./Figures/CDN_GrpSp/ImgNo1_Noise16_X_resid_CDN.eps}
		\end{minipage} 
		\begin{minipage}[b]{0.28\linewidth}
			\centering
			\includegraphics[width = 2.5cm, height = 2.5cm]{./Figures/CDN_GrpSp/ImgNo1_Noise24_X_resid_CDN.eps}
		\end{minipage} 
		\\
		% ------------------------------------------- 
		\begin{minipage}[b]{0.1\linewidth}
			\centering	% {\phantom{{\footnotesize XXX}}} 
		\end{minipage}
		\begin{minipage}[b]{0.28\linewidth}
			\centering	{\footnotesize $\sigma=8$}
		\end{minipage} 
		\begin{minipage}[b]{0.28\linewidth}
			\centering	{\footnotesize $\sigma=16$} 
		\end{minipage} 
		\begin{minipage}[b]{0.28\linewidth}
			\centering	{\footnotesize $\sigma=24$} 
		\end{minipage}
		% -------------------------------------------	
	\end{multicols}	

	\vspace{-0.8cm}

	\begin{multicols}{1}  
		\begin{minipage}[b]{0.98\linewidth}
			{\footnotesize Colorbar}
			\includegraphics[width = 16.8cm, height=0.5cm]{./Figures/Colorbar64.eps}
		\end{minipage}
	\end{multicols}	
	
	\vspace{-0.6cm}

	\caption{Visual comparison on multimodal image denoising.}
	%	 Each row represents one approach and its denoising results corresponding to different noise levels.}
	\label{Fig:DenoisedIms_1}
\end{figure*}

\begin{figure*}[th]
	\begin{multicols}{2}  
		\centering
		% ------------------------------------------- 
		% Noisy images
		\begin{minipage}[b]{0.1\linewidth}
			\centering
			{\footnotesize Input}  
		\end{minipage} 
		\begin{minipage}[b]{0.28\linewidth}
			\centering
			\includegraphics[width = 2.5cm, height = 2.5cm]{./Figures/GF/ImgNo2_Noise8_X_low.eps}
		\end{minipage} 
		\begin{minipage}[b]{0.28\linewidth}
			\centering
			\includegraphics[width = 2.5cm, height = 2.5cm]{./Figures/GF/ImgNo2_Noise16_X_low.eps}
		\end{minipage} 
		\begin{minipage}[b]{0.28\linewidth}
			\centering
			\includegraphics[width = 2.5cm, height = 2.5cm]{./Figures/GF/ImgNo2_Noise24_X_low.eps}
		\end{minipage} 
		\\
		% ------------------------------------------- 
		% JBF
		\begin{minipage}[b]{0.1\linewidth}
			\centering
			{\footnotesize JBF~\cite{kopf2007joint}} % 
		\end{minipage} 
		\begin{minipage}[b]{0.28\linewidth}
			\centering
			\includegraphics[width = 2.5cm, height = 2.5cm]{./Figures/JBF/ImgNo2_Noise8_X_JBF.eps}
		\end{minipage}  
		\begin{minipage}[b]{0.28\linewidth}
			\centering
			\includegraphics[width = 2.5cm, height = 2.5cm]{./Figures/JBF/ImgNo2_Noise16_X_JBF.eps}
		\end{minipage} 
		\begin{minipage}[b]{0.28\linewidth}
			\centering
			\includegraphics[width = 2.5cm, height = 2.5cm]{./Figures/JBF/ImgNo2_Noise24_X_JBF.eps}
		\end{minipage} 
		\\
		% ------------------------------------------- 
		% JBF
		\begin{minipage}[b]{0.1\linewidth}
			\centering
			{\footnotesize ErrMap JBF~\cite{kopf2007joint}} % 
		\end{minipage} 
		\begin{minipage}[b]{0.28\linewidth}
			\centering
			\includegraphics[width = 2.5cm, height = 2.5cm]{./Figures/JBF/ImgNo2_Noise8_X_resid_JBF.eps}
		\end{minipage} 
		\begin{minipage}[b]{0.28\linewidth}
			\centering
			\includegraphics[width = 2.5cm, height = 2.5cm]{./Figures/JBF/ImgNo2_Noise16_X_resid_JBF.eps}
		\end{minipage} 
		\begin{minipage}[b]{0.28\linewidth}
			\centering
			\includegraphics[width = 2.5cm, height = 2.5cm]{./Figures/JBF/ImgNo2_Noise24_X_resid_JBF.eps}
		\end{minipage} 
		\\
		% ------------------------------------------- 
		% GF
		\begin{minipage}[b]{0.1\linewidth}
			\centering
			{\footnotesize GF~\cite{he2013guided}}  
		\end{minipage}  
		\begin{minipage}[b]{0.28\linewidth}
			\centering
			\includegraphics[width = 2.5cm, height = 2.5cm]{./Figures/GF/ImgNo2_Noise8_X_GF.eps}
		\end{minipage} 
		\begin{minipage}[b]{0.28\linewidth}
			\centering
			\includegraphics[width = 2.5cm, height = 2.5cm]{./Figures/GF/ImgNo2_Noise16_X_GF.eps}
		\end{minipage} 
		\begin{minipage}[b]{0.28\linewidth}
			\centering
			\includegraphics[width = 2.5cm, height = 2.5cm]{./Figures/GF/ImgNo2_Noise24_X_GF.eps}
		\end{minipage} 
		\\
		% ------------------------------------------- 
		% GF
		\begin{minipage}[b]{0.1\linewidth}
			\centering
			{\footnotesize ErrMap GF~\cite{he2013guided}}  
		\end{minipage} 
		\begin{minipage}[b]{0.28\linewidth}
			\centering
			\includegraphics[width = 2.5cm, height = 2.5cm]{./Figures/GF/ImgNo2_Noise8_X_resid_GF.eps}
		\end{minipage} 
		\begin{minipage}[b]{0.28\linewidth}
			\centering
			\includegraphics[width = 2.5cm, height = 2.5cm]{./Figures/GF/ImgNo2_Noise16_X_resid_GF.eps}
		\end{minipage} 
		\begin{minipage}[b]{0.28\linewidth}
			\centering
			\includegraphics[width = 2.5cm, height = 2.5cm]{./Figures/GF/ImgNo2_Noise24_X_resid_GF.eps}
		\end{minipage} 
		\\
		% -------------------------------------------
		% SDF
		\begin{minipage}[b]{0.1\linewidth}
			\centering
			{\footnotesize SDF~\cite{ham2017robust}} %  
		\end{minipage} 
		\begin{minipage}[b]{0.28\linewidth}
			\centering
			\includegraphics[width = 2.5cm, height = 2.5cm]{./Figures/SDF/ImgNo2_Noise8_X_SDF.eps}
		\end{minipage} 
		\begin{minipage}[b]{0.28\linewidth}
			\centering
			\includegraphics[width = 2.5cm, height = 2.5cm]{./Figures/SDF/ImgNo2_Noise16_X_SDF.eps}
		\end{minipage}  
		\begin{minipage}[b]{0.28\linewidth}
			\centering
			\includegraphics[width = 2.5cm, height = 2.5cm]{./Figures/SDF/ImgNo2_Noise24_X_SDF.eps}
		\end{minipage} 
		\\
		% -------------------------------------------
		% SDF
		\begin{minipage}[b]{0.1\linewidth}
			\centering
			{\footnotesize ErrMap SDF~\cite{ham2017robust}} % 
		\end{minipage}  
		\begin{minipage}[b]{0.28\linewidth}
			\centering
			\includegraphics[width = 2.5cm, height = 2.5cm]{./Figures/SDF/ImgNo2_Noise8_X_resid_SDF.eps}
		\end{minipage} 
		\begin{minipage}[b]{0.28\linewidth}
			\centering
			\includegraphics[width = 2.5cm, height = 2.5cm]{./Figures/SDF/ImgNo2_Noise16_X_resid_SDF.eps}
		\end{minipage} 
		\begin{minipage}[b]{0.28\linewidth}
			\centering
			\includegraphics[width = 2.5cm, height = 2.5cm]{./Figures/SDF/ImgNo2_Noise24_X_resid_SDF.eps}
		\end{minipage} 
		\\
		% ------------------------------------------- 
		\begin{minipage}[b]{0.1\linewidth}
			\centering	% {\phantom{{\footnotesize XXX}}} 
		\end{minipage}
		\begin{minipage}[b]{0.28\linewidth}
			\centering	{\footnotesize $\sigma=8$}
		\end{minipage} 
		\begin{minipage}[b]{0.28\linewidth}
			\centering	{\footnotesize $\sigma=16$} 
		\end{minipage} 
		\begin{minipage}[b]{0.28\linewidth}
			\centering	{\footnotesize $\sigma=24$} 
		\end{minipage}
		\\
		%---------------------------------------------------
		% true images
		\begin{minipage}[b]{0.1\linewidth}
			\centering
			{\footnotesize Truth}  
		\end{minipage} 
		\begin{minipage}[b]{0.28\linewidth}
			\centering
			\includegraphics[width = 2.5cm, height = 2.5cm]{./Figures/GF/ImgNo2_Noise8_X_true.eps}
		\end{minipage} 
		\begin{minipage}[b]{0.28\linewidth}
			\centering
			\includegraphics[width = 2.5cm, height = 2.5cm]{./Figures/GF/ImgNo2_Noise16_X_true.eps}
		\end{minipage} 
		\begin{minipage}[b]{0.28\linewidth}
			\centering
			\includegraphics[width = 2.5cm, height = 2.5cm]{./Figures/GF/ImgNo2_Noise24_X_true.eps}
		\end{minipage} 
		\\
		% -------------------------------------------
		% JFSM
		\begin{minipage}[b]{0.1\linewidth}
			\centering
			{\footnotesize JFSM\cite{shen2015multispectral}}  
		\end{minipage}  
		\begin{minipage}[b]{0.28\linewidth}
			\centering
			\includegraphics[width = 2.5cm, height = 2.5cm]{./Figures/JFSM/ImgNo2_Noise8_X_JFSM.eps}
		\end{minipage}  
		\begin{minipage}[b]{0.28\linewidth}
			\centering
			\includegraphics[width = 2.5cm, height = 2.5cm]{./Figures/JFSM/ImgNo2_Noise16_X_JFSM.eps}
		\end{minipage} 
		\begin{minipage}[b]{0.28\linewidth}
			\centering
			\includegraphics[width = 2.5cm, height = 2.5cm]{./Figures/JFSM/ImgNo2_Noise24_X_JFSM.eps}
		\end{minipage} 
		\\
		% -------------------------------------------	
		% JFSM
		\begin{minipage}[b]{0.1\linewidth}
			\centering
			{\footnotesize ErrMap JFSM\cite{shen2015multispectral}}  
		\end{minipage} 
		\begin{minipage}[b]{0.28\linewidth}
			\centering
			\includegraphics[width = 2.5cm, height = 2.5cm]{./Figures/JFSM/ImgNo2_Noise8_X_resid_JFSM.eps}
		\end{minipage} 
		\begin{minipage}[b]{0.28\linewidth}
			\centering
			\includegraphics[width = 2.5cm, height = 2.5cm]{./Figures/JFSM/ImgNo2_Noise16_X_resid_JFSM.eps}
		\end{minipage} 
		\begin{minipage}[b]{0.28\linewidth}
			\centering
			\includegraphics[width = 2.5cm, height = 2.5cm]{./Figures/JFSM/ImgNo2_Noise24_X_resid_JFSM.eps}
		\end{minipage} 
		\\
		% -------------------------------------------
		% DJF
		\begin{minipage}[b]{0.1\linewidth}
			\centering
			{\footnotesize DJF~\cite{li2016deep}} %  
		\end{minipage} 
		\begin{minipage}[b]{0.28\linewidth}
			\centering
			\includegraphics[width = 2.5cm, height = 2.5cm]{./Figures/DJF/ImgNo2_Noise8_X_DJF.eps}
		\end{minipage} 
		\begin{minipage}[b]{0.28\linewidth}
			\centering
			\includegraphics[width = 2.5cm, height = 2.5cm]{./Figures/DJF/ImgNo2_Noise16_X_DJF.eps}
		\end{minipage} 
		\begin{minipage}[b]{0.28\linewidth}
			\centering
			\includegraphics[width = 2.5cm, height = 2.5cm]{./Figures/DJF/ImgNo2_Noise24_X_DJF.eps}
		\end{minipage} 
		\\
		% -------------------------------------------
		% DJF
		\begin{minipage}[b]{0.1\linewidth}
			\centering
			{\footnotesize ErrMap DJF~\cite{li2016deep}} %  
		\end{minipage}  
		\begin{minipage}[b]{0.28\linewidth}
			\centering
			\includegraphics[width = 2.5cm, height = 2.5cm]{./Figures/DJF/ImgNo2_Noise8_X_resid_DJF.eps}
		\end{minipage} 
		\begin{minipage}[b]{0.28\linewidth}
			\centering
			\includegraphics[width = 2.5cm, height = 2.5cm]{./Figures/DJF/ImgNo2_Noise16_X_resid_DJF.eps}
		\end{minipage} 
		\begin{minipage}[b]{0.28\linewidth}
			\centering
			\includegraphics[width = 2.5cm, height = 2.5cm]{./Figures/DJF/ImgNo2_Noise24_X_resid_DJF.eps}
		\end{minipage} 
		\\
		% -------------------------------------------
		%	% CDN with standard sparsity
		%	\begin{minipage}[b]{0.1\linewidth}
		%		\centering
		%		{\footnotesize Ours} %  
		%	\end{minipage} 
		%	\begin{minipage}[b]{0.28\linewidth}
		%		\centering
		%		\includegraphics[width = 2.5cm, height = 2.5cm]{./Figures/CDN/ImgNo2_Noise4_X_CDN.eps}
		%	\end{minipage} 
		%	\begin{minipage}[b]{0.28\linewidth}
		%		\centering
		%		\includegraphics[width = 2.5cm, height = 2.5cm]{./Figures/CDN/ImgNo2_Noise12_X_CDN.eps}
		%	\end{minipage} 
		%	\begin{minipage}[b]{0.28\linewidth}
		%		\centering
		%		\includegraphics[width = 2.5cm, height = 2.5cm]{./Figures/CDN/ImgNo2_Noise20_X_CDN.eps}
		%	\end{minipage} 
		%	\\
		% -------------------------------------------
		%	% CDN with standard sparsity
		%	\begin{minipage}[b]{0.1\linewidth}
		%		\centering
		%		{\footnotesize ErrMap Ours} %  
		%	\end{minipage} 
		%	\begin{minipage}[b]{0.28\linewidth}
		%		\centering
		%		\includegraphics[width = 2.5cm, height = 2.5cm]{./Figures/CDN/ImgNo2_Noise8_X_resid_CDN.eps}
		%	\end{minipage} 
		%	\begin{minipage}[b]{0.28\linewidth}
		%		\centering
		%		\includegraphics[width = 2.5cm, height = 2.5cm]{./Figures/CDN/ImgNo2_Noise16_X_resid_CDN.eps}
		%	\end{minipage} 
		%	\begin{minipage}[b]{0.28\linewidth}
		%		\centering
		%		\includegraphics[width = 2.5cm, height = 2.5cm]{./Figures/CDN/ImgNo2_Noise24_X_resid_CDN.eps}
		%	\end{minipage} 
		%	\\
		% -------------------------------------------
		% CDN with group sparsity
		\begin{minipage}[b]{0.1\linewidth}
			\centering
			{\footnotesize Ours+}  
		\end{minipage} 
		\begin{minipage}[b]{0.28\linewidth}
			\centering
			\includegraphics[width = 2.5cm, height = 2.5cm]{./Figures/CDN_GrpSp/ImgNo2_Noise8_X_CDN.eps}
		\end{minipage} 
		\begin{minipage}[b]{0.28\linewidth}
			\centering
			\includegraphics[width = 2.5cm, height = 2.5cm]{./Figures/CDN_GrpSp/ImgNo2_Noise16_X_CDN.eps}
		\end{minipage} 
		\begin{minipage}[b]{0.28\linewidth}
			\centering
			\includegraphics[width = 2.5cm, height = 2.5cm]{./Figures/CDN_GrpSp/ImgNo2_Noise24_X_CDN.eps}
		\end{minipage} 
		\\
		% -------------------------------------------
		% CDN with group sparsity
		\begin{minipage}[b]{0.1\linewidth}
			\centering
			{\footnotesize ErrMap Ours+}  
		\end{minipage} 
		\begin{minipage}[b]{0.28\linewidth}
			\centering
			\includegraphics[width = 2.5cm, height = 2.5cm]{./Figures/CDN_GrpSp/ImgNo2_Noise8_X_resid_CDN.eps}
		\end{minipage} 
		\begin{minipage}[b]{0.28\linewidth}
			\centering
			\includegraphics[width = 2.5cm, height = 2.5cm]{./Figures/CDN_GrpSp/ImgNo2_Noise16_X_resid_CDN.eps}
		\end{minipage} 
		\begin{minipage}[b]{0.28\linewidth}
			\centering
			\includegraphics[width = 2.5cm, height = 2.5cm]{./Figures/CDN_GrpSp/ImgNo2_Noise24_X_resid_CDN.eps}
		\end{minipage} 
		\\
		% ------------------------------------------- 
		\begin{minipage}[b]{0.1\linewidth}
			\centering	% {\phantom{{\footnotesize XXX}}} 
		\end{minipage}
		\begin{minipage}[b]{0.28\linewidth}
			\centering	{\footnotesize $\sigma=8$}
		\end{minipage} 
		\begin{minipage}[b]{0.28\linewidth}
			\centering	{\footnotesize $\sigma=16$} 
		\end{minipage} 
		\begin{minipage}[b]{0.28\linewidth}
			\centering	{\footnotesize $\sigma=24$} 
		\end{minipage}
		% -------------------------------------------	
	\end{multicols}	
	
	\vspace{-0.8cm}
	
	\begin{multicols}{1}  
		\begin{minipage}[b]{0.98\linewidth}
			{\footnotesize Colorbar}
			\includegraphics[width = 16.8cm, height=0.5cm]{./Figures/Colorbar64.eps}
		\end{minipage}
	\end{multicols}	
	
	\vspace{-0.6cm}
	
	\caption{Visual comparison on multimodal image denoising.}
	%	 Each row represents one approach and its denoising results corresponding to different noise levels.}
	\label{Fig:DenoisedIms_2}
\end{figure*}

%%=====================================================================================

%% image No3 -- denoised images for only 3 noise levels
\begin{figure*}[th]
	\begin{multicols}{2}  
		\centering
		% ------------------------------------------- 
		% Noisy images
		\begin{minipage}[b]{0.1\linewidth}
			\centering
			{\footnotesize Input}  
		\end{minipage} 
		\begin{minipage}[b]{0.28\linewidth}
			\centering
			\includegraphics[width = 2.5cm, height = 2.5cm]{./Figures/GF/ImgNo3_Noise8_X_low.eps}
		\end{minipage} 
		\begin{minipage}[b]{0.28\linewidth}
			\centering
			\includegraphics[width = 2.5cm, height = 2.5cm]{./Figures/GF/ImgNo3_Noise16_X_low.eps}
		\end{minipage} 
		\begin{minipage}[b]{0.28\linewidth}
			\centering
			\includegraphics[width = 2.5cm, height = 2.5cm]{./Figures/GF/ImgNo3_Noise24_X_low.eps}
		\end{minipage} 
		\\
		% ------------------------------------------- 
		% JBF
		\begin{minipage}[b]{0.1\linewidth}
			\centering
			{\footnotesize JBF~\cite{kopf2007joint}} % 
		\end{minipage} 
		\begin{minipage}[b]{0.28\linewidth}
			\centering
			\includegraphics[width = 2.5cm, height = 2.5cm]{./Figures/JBF/ImgNo3_Noise8_X_JBF.eps}
		\end{minipage}  
		\begin{minipage}[b]{0.28\linewidth}
			\centering
			\includegraphics[width = 2.5cm, height = 2.5cm]{./Figures/JBF/ImgNo3_Noise16_X_JBF.eps}
		\end{minipage} 
		\begin{minipage}[b]{0.28\linewidth}
			\centering
			\includegraphics[width = 2.5cm, height = 2.5cm]{./Figures/JBF/ImgNo3_Noise24_X_JBF.eps}
		\end{minipage} 
		\\
		% ------------------------------------------- 
		% JBF
		\begin{minipage}[b]{0.1\linewidth}
			\centering
			{\footnotesize ErrMap JBF~\cite{kopf2007joint}} % 
		\end{minipage} 
		\begin{minipage}[b]{0.28\linewidth}
			\centering
			\includegraphics[width = 2.5cm, height = 2.5cm]{./Figures/JBF/ImgNo3_Noise8_X_resid_JBF.eps}
		\end{minipage} 
		\begin{minipage}[b]{0.28\linewidth}
			\centering
			\includegraphics[width = 2.5cm, height = 2.5cm]{./Figures/JBF/ImgNo3_Noise16_X_resid_JBF.eps}
		\end{minipage} 
		\begin{minipage}[b]{0.28\linewidth}
			\centering
			\includegraphics[width = 2.5cm, height = 2.5cm]{./Figures/JBF/ImgNo3_Noise24_X_resid_JBF.eps}
		\end{minipage} 
		\\
		% ------------------------------------------- 
		% GF
		\begin{minipage}[b]{0.1\linewidth}
			\centering
			{\footnotesize GF~\cite{he2013guided}}  
		\end{minipage}  
		\begin{minipage}[b]{0.28\linewidth}
			\centering
			\includegraphics[width = 2.5cm, height = 2.5cm]{./Figures/GF/ImgNo3_Noise8_X_GF.eps}
		\end{minipage} 
		\begin{minipage}[b]{0.28\linewidth}
			\centering
			\includegraphics[width = 2.5cm, height = 2.5cm]{./Figures/GF/ImgNo3_Noise16_X_GF.eps}
		\end{minipage} 
		\begin{minipage}[b]{0.28\linewidth}
			\centering
			\includegraphics[width = 2.5cm, height = 2.5cm]{./Figures/GF/ImgNo3_Noise24_X_GF.eps}
		\end{minipage} 
		\\
		% ------------------------------------------- 
		% GF
		\begin{minipage}[b]{0.1\linewidth}
			\centering
			{\footnotesize ErrMap GF~\cite{he2013guided}}  
		\end{minipage} 
		\begin{minipage}[b]{0.28\linewidth}
			\centering
			\includegraphics[width = 2.5cm, height = 2.5cm]{./Figures/GF/ImgNo3_Noise8_X_resid_GF.eps}
		\end{minipage} 
		\begin{minipage}[b]{0.28\linewidth}
			\centering
			\includegraphics[width = 2.5cm, height = 2.5cm]{./Figures/GF/ImgNo3_Noise16_X_resid_GF.eps}
		\end{minipage} 
		\begin{minipage}[b]{0.28\linewidth}
			\centering
			\includegraphics[width = 2.5cm, height = 2.5cm]{./Figures/GF/ImgNo3_Noise24_X_resid_GF.eps}
		\end{minipage} 
		\\
		% -------------------------------------------
		% SDF
		\begin{minipage}[b]{0.1\linewidth}
			\centering
			{\footnotesize SDF~\cite{ham2017robust}} %  
		\end{minipage} 
		\begin{minipage}[b]{0.28\linewidth}
			\centering
			\includegraphics[width = 2.5cm, height = 2.5cm]{./Figures/SDF/ImgNo3_Noise8_X_SDF.eps}
		\end{minipage} 
		\begin{minipage}[b]{0.28\linewidth}
			\centering
			\includegraphics[width = 2.5cm, height = 2.5cm]{./Figures/SDF/ImgNo3_Noise16_X_SDF.eps}
		\end{minipage}  
		\begin{minipage}[b]{0.28\linewidth}
			\centering
			\includegraphics[width = 2.5cm, height = 2.5cm]{./Figures/SDF/ImgNo3_Noise24_X_SDF.eps}
		\end{minipage} 
		\\
		% -------------------------------------------
		% SDF
		\begin{minipage}[b]{0.1\linewidth}
			\centering
			{\footnotesize ErrMap SDF~\cite{ham2017robust}} % 
		\end{minipage}  
		\begin{minipage}[b]{0.28\linewidth}
			\centering
			\includegraphics[width = 2.5cm, height = 2.5cm]{./Figures/SDF/ImgNo3_Noise8_X_resid_SDF.eps}
		\end{minipage} 
		\begin{minipage}[b]{0.28\linewidth}
			\centering
			\includegraphics[width = 2.5cm, height = 2.5cm]{./Figures/SDF/ImgNo3_Noise16_X_resid_SDF.eps}
		\end{minipage} 
		\begin{minipage}[b]{0.28\linewidth}
			\centering
			\includegraphics[width = 2.5cm, height = 2.5cm]{./Figures/SDF/ImgNo3_Noise24_X_resid_SDF.eps}
		\end{minipage} 
		\\
		% ------------------------------------------- 
		\begin{minipage}[b]{0.1\linewidth}
			\centering	% {\phantom{{\footnotesize XXX}}} 
		\end{minipage}
		\begin{minipage}[b]{0.28\linewidth}
			\centering	{\footnotesize $\sigma=8$}
		\end{minipage} 
		\begin{minipage}[b]{0.28\linewidth}
			\centering	{\footnotesize $\sigma=16$} 
		\end{minipage} 
		\begin{minipage}[b]{0.28\linewidth}
			\centering	{\footnotesize $\sigma=24$} 
		\end{minipage}
		\\
		%---------------------------------------------------
		% true images
		\begin{minipage}[b]{0.1\linewidth}
			\centering
			{\footnotesize Truth}  
		\end{minipage} 
		\begin{minipage}[b]{0.28\linewidth}
			\centering
			\includegraphics[width = 2.5cm, height = 2.5cm]{./Figures/GF/ImgNo3_Noise8_X_true.eps}
		\end{minipage} 
		\begin{minipage}[b]{0.28\linewidth}
			\centering
			\includegraphics[width = 2.5cm, height = 2.5cm]{./Figures/GF/ImgNo3_Noise16_X_true.eps}
		\end{minipage} 
		\begin{minipage}[b]{0.28\linewidth}
			\centering
			\includegraphics[width = 2.5cm, height = 2.5cm]{./Figures/GF/ImgNo3_Noise24_X_true.eps}
		\end{minipage} 
		\\
		% -------------------------------------------
		% JFSM
		\begin{minipage}[b]{0.1\linewidth}
			\centering
			{\footnotesize JFSM\cite{shen2015multispectral}}  
		\end{minipage}  
		\begin{minipage}[b]{0.28\linewidth}
			\centering
			\includegraphics[width = 2.5cm, height = 2.5cm]{./Figures/JFSM/ImgNo3_Noise8_X_JFSM.eps}
		\end{minipage}  
		\begin{minipage}[b]{0.28\linewidth}
			\centering
			\includegraphics[width = 2.5cm, height = 2.5cm]{./Figures/JFSM/ImgNo3_Noise16_X_JFSM.eps}
		\end{minipage} 
		\begin{minipage}[b]{0.28\linewidth}
			\centering
			\includegraphics[width = 2.5cm, height = 2.5cm]{./Figures/JFSM/ImgNo3_Noise24_X_JFSM.eps}
		\end{minipage} 
		\\
		% -------------------------------------------	
		% JFSM
		\begin{minipage}[b]{0.1\linewidth}
			\centering
			{\footnotesize ErrMap JFSM\cite{shen2015multispectral}}  
		\end{minipage} 
		\begin{minipage}[b]{0.28\linewidth}
			\centering
			\includegraphics[width = 2.5cm, height = 2.5cm]{./Figures/JFSM/ImgNo3_Noise8_X_resid_JFSM.eps}
		\end{minipage} 
		\begin{minipage}[b]{0.28\linewidth}
			\centering
			\includegraphics[width = 2.5cm, height = 2.5cm]{./Figures/JFSM/ImgNo3_Noise16_X_resid_JFSM.eps}
		\end{minipage} 
		\begin{minipage}[b]{0.28\linewidth}
			\centering
			\includegraphics[width = 2.5cm, height = 2.5cm]{./Figures/JFSM/ImgNo3_Noise24_X_resid_JFSM.eps}
		\end{minipage} 
		\\
		% -------------------------------------------
		% DJF
		\begin{minipage}[b]{0.1\linewidth}
			\centering
			{\footnotesize DJF~\cite{li2016deep}} %  
		\end{minipage} 
		\begin{minipage}[b]{0.28\linewidth}
			\centering
			\includegraphics[width = 2.5cm, height = 2.5cm]{./Figures/DJF/ImgNo3_Noise8_X_DJF.eps}
		\end{minipage} 
		\begin{minipage}[b]{0.28\linewidth}
			\centering
			\includegraphics[width = 2.5cm, height = 2.5cm]{./Figures/DJF/ImgNo3_Noise16_X_DJF.eps}
		\end{minipage} 
		\begin{minipage}[b]{0.28\linewidth}
			\centering
			\includegraphics[width = 2.5cm, height = 2.5cm]{./Figures/DJF/ImgNo3_Noise24_X_DJF.eps}
		\end{minipage} 
		\\
		% -------------------------------------------
		% DJF
		\begin{minipage}[b]{0.1\linewidth}
			\centering
			{\footnotesize ErrMap DJF~\cite{li2016deep}} %  
		\end{minipage}  
		\begin{minipage}[b]{0.28\linewidth}
			\centering
			\includegraphics[width = 2.5cm, height = 2.5cm]{./Figures/DJF/ImgNo3_Noise8_X_resid_DJF.eps}
		\end{minipage} 
		\begin{minipage}[b]{0.28\linewidth}
			\centering
			\includegraphics[width = 2.5cm, height = 2.5cm]{./Figures/DJF/ImgNo3_Noise16_X_resid_DJF.eps}
		\end{minipage} 
		\begin{minipage}[b]{0.28\linewidth}
			\centering
			\includegraphics[width = 2.5cm, height = 2.5cm]{./Figures/DJF/ImgNo3_Noise24_X_resid_DJF.eps}
		\end{minipage} 
		\\
		% -------------------------------------------
		%	% CDN with standard sparsity
		%	\begin{minipage}[b]{0.1\linewidth}
		%		\centering
		%		{\footnotesize Ours} %  
		%	\end{minipage} 
		%	\begin{minipage}[b]{0.28\linewidth}
		%		\centering
		%		\includegraphics[width = 2.5cm, height = 2.5cm]{./Figures/CDN/ImgNo3_Noise4_X_CDN.eps}
		%	\end{minipage} 
		%	\begin{minipage}[b]{0.28\linewidth}
		%		\centering
		%		\includegraphics[width = 2.5cm, height = 2.5cm]{./Figures/CDN/ImgNo3_Noise12_X_CDN.eps}
		%	\end{minipage} 
		%	\begin{minipage}[b]{0.28\linewidth}
		%		\centering
		%		\includegraphics[width = 2.5cm, height = 2.5cm]{./Figures/CDN/ImgNo3_Noise20_X_CDN.eps}
		%	\end{minipage} 
		%	\\
		% -------------------------------------------
		%	% CDN with standard sparsity
		%	\begin{minipage}[b]{0.1\linewidth}
		%		\centering
		%		{\footnotesize ErrMap Ours} %  
		%	\end{minipage} 
		%	\begin{minipage}[b]{0.28\linewidth}
		%		\centering
		%		\includegraphics[width = 2.5cm, height = 2.5cm]{./Figures/CDN/ImgNo3_Noise8_X_resid_CDN.eps}
		%	\end{minipage} 
		%	\begin{minipage}[b]{0.28\linewidth}
		%		\centering
		%		\includegraphics[width = 2.5cm, height = 2.5cm]{./Figures/CDN/ImgNo3_Noise16_X_resid_CDN.eps}
		%	\end{minipage} 
		%	\begin{minipage}[b]{0.28\linewidth}
		%		\centering
		%		\includegraphics[width = 2.5cm, height = 2.5cm]{./Figures/CDN/ImgNo3_Noise24_X_resid_CDN.eps}
		%	\end{minipage} 
		%	\\
		% -------------------------------------------
		% CDN with group sparsity
		\begin{minipage}[b]{0.1\linewidth}
			\centering
			{\footnotesize Ours+}  
		\end{minipage} 
		\begin{minipage}[b]{0.28\linewidth}
			\centering
			\includegraphics[width = 2.5cm, height = 2.5cm]{./Figures/CDN_GrpSp/ImgNo3_Noise8_X_CDN.eps}
		\end{minipage} 
		\begin{minipage}[b]{0.28\linewidth}
			\centering
			\includegraphics[width = 2.5cm, height = 2.5cm]{./Figures/CDN_GrpSp/ImgNo3_Noise16_X_CDN.eps}
		\end{minipage} 
		\begin{minipage}[b]{0.28\linewidth}
			\centering
			\includegraphics[width = 2.5cm, height = 2.5cm]{./Figures/CDN_GrpSp/ImgNo3_Noise24_X_CDN.eps}
		\end{minipage} 
		\\
		% -------------------------------------------
		% CDN with group sparsity
		\begin{minipage}[b]{0.1\linewidth}
			\centering
			{\footnotesize ErrMap Ours+}  
		\end{minipage} 
		\begin{minipage}[b]{0.28\linewidth}
			\centering
			\includegraphics[width = 2.5cm, height = 2.5cm]{./Figures/CDN_GrpSp/ImgNo3_Noise8_X_resid_CDN.eps}
		\end{minipage} 
		\begin{minipage}[b]{0.28\linewidth}
			\centering
			\includegraphics[width = 2.5cm, height = 2.5cm]{./Figures/CDN_GrpSp/ImgNo3_Noise16_X_resid_CDN.eps}
		\end{minipage} 
		\begin{minipage}[b]{0.28\linewidth}
			\centering
			\includegraphics[width = 2.5cm, height = 2.5cm]{./Figures/CDN_GrpSp/ImgNo3_Noise24_X_resid_CDN.eps}
		\end{minipage} 
		\\
		% ------------------------------------------- 
		\begin{minipage}[b]{0.1\linewidth}
			\centering	% {\phantom{{\footnotesize XXX}}} 
		\end{minipage}
		\begin{minipage}[b]{0.28\linewidth}
			\centering	{\footnotesize $\sigma=8$}
		\end{minipage} 
		\begin{minipage}[b]{0.28\linewidth}
			\centering	{\footnotesize $\sigma=16$} 
		\end{minipage} 
		\begin{minipage}[b]{0.28\linewidth}
			\centering	{\footnotesize $\sigma=24$} 
		\end{minipage}
		% -------------------------------------------	
	\end{multicols}	
	
	\vspace{-0.8cm}
	
	\begin{multicols}{1}  
		\begin{minipage}[b]{0.98\linewidth}
			{\footnotesize Colorbar}
			\includegraphics[width = 16.8cm, height=0.5cm]{./Figures/Colorbar64.eps}
		\end{minipage}
	\end{multicols}	
	
	\vspace{-0.6cm}
	
	\caption{Visual comparison on multimodal image denoising.}
	%	 Each row represents one approach and its denoising results corresponding to different noise levels.}
	\label{Fig:DenoisedIms_3}
\end{figure*}

%%======================================================================================

%% image No4 -- denoised images for only 3 noise levels
\begin{figure*}[th]
	\begin{multicols}{2}  
		\centering
		% ------------------------------------------- 
		% Noisy images
		\begin{minipage}[b]{0.1\linewidth}
			\centering
			{\footnotesize Input}  
		\end{minipage} 
		\begin{minipage}[b]{0.28\linewidth}
			\centering
			\includegraphics[width = 2.5cm, height = 2.5cm]{./Figures/GF/ImgNo4_Noise8_X_low.eps}
		\end{minipage} 
		\begin{minipage}[b]{0.28\linewidth}
			\centering
			\includegraphics[width = 2.5cm, height = 2.5cm]{./Figures/GF/ImgNo4_Noise16_X_low.eps}
		\end{minipage} 
		\begin{minipage}[b]{0.28\linewidth}
			\centering
			\includegraphics[width = 2.5cm, height = 2.5cm]{./Figures/GF/ImgNo4_Noise24_X_low.eps}
		\end{minipage} 
		\\
		% ------------------------------------------- 
		% JBF
		\begin{minipage}[b]{0.1\linewidth}
			\centering
			{\footnotesize JBF~\cite{kopf2007joint}} % 
		\end{minipage} 
		\begin{minipage}[b]{0.28\linewidth}
			\centering
			\includegraphics[width = 2.5cm, height = 2.5cm]{./Figures/JBF/ImgNo4_Noise8_X_JBF.eps}
		\end{minipage}  
		\begin{minipage}[b]{0.28\linewidth}
			\centering
			\includegraphics[width = 2.5cm, height = 2.5cm]{./Figures/JBF/ImgNo4_Noise16_X_JBF.eps}
		\end{minipage} 
		\begin{minipage}[b]{0.28\linewidth}
			\centering
			\includegraphics[width = 2.5cm, height = 2.5cm]{./Figures/JBF/ImgNo4_Noise24_X_JBF.eps}
		\end{minipage} 
		\\
		% ------------------------------------------- 
		% JBF
		\begin{minipage}[b]{0.1\linewidth}
			\centering
			{\footnotesize ErrMap JBF~\cite{kopf2007joint}} % 
		\end{minipage} 
		\begin{minipage}[b]{0.28\linewidth}
			\centering
			\includegraphics[width = 2.5cm, height = 2.5cm]{./Figures/JBF/ImgNo4_Noise8_X_resid_JBF.eps}
		\end{minipage} 
		\begin{minipage}[b]{0.28\linewidth}
			\centering
			\includegraphics[width = 2.5cm, height = 2.5cm]{./Figures/JBF/ImgNo4_Noise16_X_resid_JBF.eps}
		\end{minipage} 
		\begin{minipage}[b]{0.28\linewidth}
			\centering
			\includegraphics[width = 2.5cm, height = 2.5cm]{./Figures/JBF/ImgNo4_Noise24_X_resid_JBF.eps}
		\end{minipage} 
		\\
		% ------------------------------------------- 
		% GF
		\begin{minipage}[b]{0.1\linewidth}
			\centering
			{\footnotesize GF~\cite{he2013guided}}  
		\end{minipage}  
		\begin{minipage}[b]{0.28\linewidth}
			\centering
			\includegraphics[width = 2.5cm, height = 2.5cm]{./Figures/GF/ImgNo4_Noise8_X_GF.eps}
		\end{minipage} 
		\begin{minipage}[b]{0.28\linewidth}
			\centering
			\includegraphics[width = 2.5cm, height = 2.5cm]{./Figures/GF/ImgNo4_Noise16_X_GF.eps}
		\end{minipage} 
		\begin{minipage}[b]{0.28\linewidth}
			\centering
			\includegraphics[width = 2.5cm, height = 2.5cm]{./Figures/GF/ImgNo4_Noise24_X_GF.eps}
		\end{minipage} 
		\\
		% ------------------------------------------- 
		% GF
		\begin{minipage}[b]{0.1\linewidth}
			\centering
			{\footnotesize ErrMap GF~\cite{he2013guided}}  
		\end{minipage} 
		\begin{minipage}[b]{0.28\linewidth}
			\centering
			\includegraphics[width = 2.5cm, height = 2.5cm]{./Figures/GF/ImgNo4_Noise8_X_resid_GF.eps}
		\end{minipage} 
		\begin{minipage}[b]{0.28\linewidth}
			\centering
			\includegraphics[width = 2.5cm, height = 2.5cm]{./Figures/GF/ImgNo4_Noise16_X_resid_GF.eps}
		\end{minipage} 
		\begin{minipage}[b]{0.28\linewidth}
			\centering
			\includegraphics[width = 2.5cm, height = 2.5cm]{./Figures/GF/ImgNo4_Noise24_X_resid_GF.eps}
		\end{minipage} 
		\\
		% -------------------------------------------
		% SDF
		\begin{minipage}[b]{0.1\linewidth}
			\centering
			{\footnotesize SDF~\cite{ham2017robust}} %  
		\end{minipage} 
		\begin{minipage}[b]{0.28\linewidth}
			\centering
			\includegraphics[width = 2.5cm, height = 2.5cm]{./Figures/SDF/ImgNo4_Noise8_X_SDF.eps}
		\end{minipage} 
		\begin{minipage}[b]{0.28\linewidth}
			\centering
			\includegraphics[width = 2.5cm, height = 2.5cm]{./Figures/SDF/ImgNo4_Noise16_X_SDF.eps}
		\end{minipage}  
		\begin{minipage}[b]{0.28\linewidth}
			\centering
			\includegraphics[width = 2.5cm, height = 2.5cm]{./Figures/SDF/ImgNo4_Noise24_X_SDF.eps}
		\end{minipage} 
		\\
		% -------------------------------------------
		% SDF
		\begin{minipage}[b]{0.1\linewidth}
			\centering
			{\footnotesize ErrMap SDF~\cite{ham2017robust}} % 
		\end{minipage}  
		\begin{minipage}[b]{0.28\linewidth}
			\centering
			\includegraphics[width = 2.5cm, height = 2.5cm]{./Figures/SDF/ImgNo4_Noise8_X_resid_SDF.eps}
		\end{minipage} 
		\begin{minipage}[b]{0.28\linewidth}
			\centering
			\includegraphics[width = 2.5cm, height = 2.5cm]{./Figures/SDF/ImgNo4_Noise16_X_resid_SDF.eps}
		\end{minipage} 
		\begin{minipage}[b]{0.28\linewidth}
			\centering
			\includegraphics[width = 2.5cm, height = 2.5cm]{./Figures/SDF/ImgNo4_Noise24_X_resid_SDF.eps}
		\end{minipage} 
		\\
		% ------------------------------------------- 
		\begin{minipage}[b]{0.1\linewidth}
			\centering	% {\phantom{{\footnotesize XXX}}} 
		\end{minipage}
		\begin{minipage}[b]{0.28\linewidth}
			\centering	{\footnotesize $\sigma=8$}
		\end{minipage} 
		\begin{minipage}[b]{0.28\linewidth}
			\centering	{\footnotesize $\sigma=16$} 
		\end{minipage} 
		\begin{minipage}[b]{0.28\linewidth}
			\centering	{\footnotesize $\sigma=24$} 
		\end{minipage}
		\\
		%---------------------------------------------------
		% true images
		\begin{minipage}[b]{0.1\linewidth}
			\centering
			{\footnotesize Truth}  
		\end{minipage} 
		\begin{minipage}[b]{0.28\linewidth}
			\centering
			\includegraphics[width = 2.5cm, height = 2.5cm]{./Figures/GF/ImgNo4_Noise8_X_true.eps}
		\end{minipage} 
		\begin{minipage}[b]{0.28\linewidth}
			\centering
			\includegraphics[width = 2.5cm, height = 2.5cm]{./Figures/GF/ImgNo4_Noise16_X_true.eps}
		\end{minipage} 
		\begin{minipage}[b]{0.28\linewidth}
			\centering
			\includegraphics[width = 2.5cm, height = 2.5cm]{./Figures/GF/ImgNo4_Noise24_X_true.eps}
		\end{minipage} 
		\\
		% -------------------------------------------
		% JFSM
		\begin{minipage}[b]{0.1\linewidth}
			\centering
			{\footnotesize JFSM\cite{shen2015multispectral}}  
		\end{minipage}  
		\begin{minipage}[b]{0.28\linewidth}
			\centering
			\includegraphics[width = 2.5cm, height = 2.5cm]{./Figures/JFSM/ImgNo4_Noise8_X_JFSM.eps}
		\end{minipage}  
		\begin{minipage}[b]{0.28\linewidth}
			\centering
			\includegraphics[width = 2.5cm, height = 2.5cm]{./Figures/JFSM/ImgNo4_Noise16_X_JFSM.eps}
		\end{minipage} 
		\begin{minipage}[b]{0.28\linewidth}
			\centering
			\includegraphics[width = 2.5cm, height = 2.5cm]{./Figures/JFSM/ImgNo4_Noise24_X_JFSM.eps}
		\end{minipage} 
		\\
		% -------------------------------------------	
		% JFSM
		\begin{minipage}[b]{0.1\linewidth}
			\centering
			{\footnotesize ErrMap JFSM\cite{shen2015multispectral}}  
		\end{minipage} 
		\begin{minipage}[b]{0.28\linewidth}
			\centering
			\includegraphics[width = 2.5cm, height = 2.5cm]{./Figures/JFSM/ImgNo4_Noise8_X_resid_JFSM.eps}
		\end{minipage} 
		\begin{minipage}[b]{0.28\linewidth}
			\centering
			\includegraphics[width = 2.5cm, height = 2.5cm]{./Figures/JFSM/ImgNo4_Noise16_X_resid_JFSM.eps}
		\end{minipage} 
		\begin{minipage}[b]{0.28\linewidth}
			\centering
			\includegraphics[width = 2.5cm, height = 2.5cm]{./Figures/JFSM/ImgNo4_Noise24_X_resid_JFSM.eps}
		\end{minipage} 
		\\
		% -------------------------------------------
		% DJF
		\begin{minipage}[b]{0.1\linewidth}
			\centering
			{\footnotesize DJF~\cite{li2016deep}} %  
		\end{minipage} 
		\begin{minipage}[b]{0.28\linewidth}
			\centering
			\includegraphics[width = 2.5cm, height = 2.5cm]{./Figures/DJF/ImgNo4_Noise8_X_DJF.eps}
		\end{minipage} 
		\begin{minipage}[b]{0.28\linewidth}
			\centering
			\includegraphics[width = 2.5cm, height = 2.5cm]{./Figures/DJF/ImgNo4_Noise16_X_DJF.eps}
		\end{minipage} 
		\begin{minipage}[b]{0.28\linewidth}
			\centering
			\includegraphics[width = 2.5cm, height = 2.5cm]{./Figures/DJF/ImgNo4_Noise24_X_DJF.eps}
		\end{minipage} 
		\\
		% -------------------------------------------
		% DJF
		\begin{minipage}[b]{0.1\linewidth}
			\centering
			{\footnotesize ErrMap DJF~\cite{li2016deep}} %  
		\end{minipage}  
		\begin{minipage}[b]{0.28\linewidth}
			\centering
			\includegraphics[width = 2.5cm, height = 2.5cm]{./Figures/DJF/ImgNo4_Noise8_X_resid_DJF.eps}
		\end{minipage} 
		\begin{minipage}[b]{0.28\linewidth}
			\centering
			\includegraphics[width = 2.5cm, height = 2.5cm]{./Figures/DJF/ImgNo4_Noise16_X_resid_DJF.eps}
		\end{minipage} 
		\begin{minipage}[b]{0.28\linewidth}
			\centering
			\includegraphics[width = 2.5cm, height = 2.5cm]{./Figures/DJF/ImgNo4_Noise24_X_resid_DJF.eps}
		\end{minipage} 
		\\
		% -------------------------------------------
		%	% CDN with standard sparsity
		%	\begin{minipage}[b]{0.1\linewidth}
		%		\centering
		%		{\footnotesize Ours} %  
		%	\end{minipage} 
		%	\begin{minipage}[b]{0.28\linewidth}
		%		\centering
		%		\includegraphics[width = 2.5cm, height = 2.5cm]{./Figures/CDN/ImgNo4_Noise4_X_CDN.eps}
		%	\end{minipage} 
		%	\begin{minipage}[b]{0.28\linewidth}
		%		\centering
		%		\includegraphics[width = 2.5cm, height = 2.5cm]{./Figures/CDN/ImgNo4_Noise12_X_CDN.eps}
		%	\end{minipage} 
		%	\begin{minipage}[b]{0.28\linewidth}
		%		\centering
		%		\includegraphics[width = 2.5cm, height = 2.5cm]{./Figures/CDN/ImgNo4_Noise20_X_CDN.eps}
		%	\end{minipage} 
		%	\\
		% -------------------------------------------
		%	% CDN with standard sparsity
		%	\begin{minipage}[b]{0.1\linewidth}
		%		\centering
		%		{\footnotesize ErrMap Ours} %  
		%	\end{minipage} 
		%	\begin{minipage}[b]{0.28\linewidth}
		%		\centering
		%		\includegraphics[width = 2.5cm, height = 2.5cm]{./Figures/CDN/ImgNo4_Noise8_X_resid_CDN.eps}
		%	\end{minipage} 
		%	\begin{minipage}[b]{0.28\linewidth}
		%		\centering
		%		\includegraphics[width = 2.5cm, height = 2.5cm]{./Figures/CDN/ImgNo4_Noise16_X_resid_CDN.eps}
		%	\end{minipage} 
		%	\begin{minipage}[b]{0.28\linewidth}
		%		\centering
		%		\includegraphics[width = 2.5cm, height = 2.5cm]{./Figures/CDN/ImgNo4_Noise24_X_resid_CDN.eps}
		%	\end{minipage} 
		%	\\
		% -------------------------------------------
		% CDN with group sparsity
		\begin{minipage}[b]{0.1\linewidth}
			\centering
			{\footnotesize Ours+}  
		\end{minipage} 
		\begin{minipage}[b]{0.28\linewidth}
			\centering
			\includegraphics[width = 2.5cm, height = 2.5cm]{./Figures/CDN_GrpSp/ImgNo4_Noise8_X_CDN.eps}
		\end{minipage} 
		\begin{minipage}[b]{0.28\linewidth}
			\centering
			\includegraphics[width = 2.5cm, height = 2.5cm]{./Figures/CDN_GrpSp/ImgNo4_Noise16_X_CDN.eps}
		\end{minipage} 
		\begin{minipage}[b]{0.28\linewidth}
			\centering
			\includegraphics[width = 2.5cm, height = 2.5cm]{./Figures/CDN_GrpSp/ImgNo4_Noise24_X_CDN.eps}
		\end{minipage} 
		\\
		% -------------------------------------------
		% CDN with group sparsity
		\begin{minipage}[b]{0.1\linewidth}
			\centering
			{\footnotesize ErrMap Ours+}  
		\end{minipage} 
		\begin{minipage}[b]{0.28\linewidth}
			\centering
			\includegraphics[width = 2.5cm, height = 2.5cm]{./Figures/CDN_GrpSp/ImgNo4_Noise8_X_resid_CDN.eps}
		\end{minipage} 
		\begin{minipage}[b]{0.28\linewidth}
			\centering
			\includegraphics[width = 2.5cm, height = 2.5cm]{./Figures/CDN_GrpSp/ImgNo4_Noise16_X_resid_CDN.eps}
		\end{minipage} 
		\begin{minipage}[b]{0.28\linewidth}
			\centering
			\includegraphics[width = 2.5cm, height = 2.5cm]{./Figures/CDN_GrpSp/ImgNo4_Noise24_X_resid_CDN.eps}
		\end{minipage} 
		\\
		% ------------------------------------------- 
		\begin{minipage}[b]{0.1\linewidth}
			\centering	% {\phantom{{\footnotesize XXX}}} 
		\end{minipage}
		\begin{minipage}[b]{0.28\linewidth}
			\centering	{\footnotesize $\sigma=8$}
		\end{minipage} 
		\begin{minipage}[b]{0.28\linewidth}
			\centering	{\footnotesize $\sigma=16$} 
		\end{minipage} 
		\begin{minipage}[b]{0.28\linewidth}
			\centering	{\footnotesize $\sigma=24$} 
		\end{minipage}
		% -------------------------------------------	
	\end{multicols}	
	
	\vspace{-0.8cm}
	
	\begin{multicols}{1}  
		\begin{minipage}[b]{0.98\linewidth}
			{\footnotesize Colorbar}
			\includegraphics[width = 16.8cm, height=0.5cm]{./Figures/Colorbar64.eps}
		\end{minipage}
	\end{multicols}	
	
	\vspace{-0.6cm}
	
	\caption{Visual comparison on multimodal image denoising.}
	%	 Each row represents one approach and its denoising results corresponding to different noise levels.}
	\label{Fig:DenoisedIms_4}
\end{figure*}

%%==========================================================================================

%% image No5 -- denoised images for only 3 noise levels
\begin{figure*}[th]
	\begin{multicols}{2}  
		\centering
		% ------------------------------------------- 
		% Noisy images
		\begin{minipage}[b]{0.1\linewidth}
			\centering
			{\footnotesize Input}  
		\end{minipage} 
		\begin{minipage}[b]{0.28\linewidth}
			\centering
			\includegraphics[width = 2.5cm, height = 2.5cm]{./Figures/GF/ImgNo5_Noise8_X_low.eps}
		\end{minipage} 
		\begin{minipage}[b]{0.28\linewidth}
			\centering
			\includegraphics[width = 2.5cm, height = 2.5cm]{./Figures/GF/ImgNo5_Noise16_X_low.eps}
		\end{minipage} 
		\begin{minipage}[b]{0.28\linewidth}
			\centering
			\includegraphics[width = 2.5cm, height = 2.5cm]{./Figures/GF/ImgNo5_Noise24_X_low.eps}
		\end{minipage} 
		\\
		% ------------------------------------------- 
		% JBF
		\begin{minipage}[b]{0.1\linewidth}
			\centering
			{\footnotesize JBF~\cite{kopf2007joint}} % 
		\end{minipage} 
		\begin{minipage}[b]{0.28\linewidth}
			\centering
			\includegraphics[width = 2.5cm, height = 2.5cm]{./Figures/JBF/ImgNo5_Noise8_X_JBF.eps}
		\end{minipage}  
		\begin{minipage}[b]{0.28\linewidth}
			\centering
			\includegraphics[width = 2.5cm, height = 2.5cm]{./Figures/JBF/ImgNo5_Noise16_X_JBF.eps}
		\end{minipage} 
		\begin{minipage}[b]{0.28\linewidth}
			\centering
			\includegraphics[width = 2.5cm, height = 2.5cm]{./Figures/JBF/ImgNo5_Noise24_X_JBF.eps}
		\end{minipage} 
		\\
		% ------------------------------------------- 
		% JBF
		\begin{minipage}[b]{0.1\linewidth}
			\centering
			{\footnotesize ErrMap JBF~\cite{kopf2007joint}} % 
		\end{minipage} 
		\begin{minipage}[b]{0.28\linewidth}
			\centering
			\includegraphics[width = 2.5cm, height = 2.5cm]{./Figures/JBF/ImgNo5_Noise8_X_resid_JBF.eps}
		\end{minipage} 
		\begin{minipage}[b]{0.28\linewidth}
			\centering
			\includegraphics[width = 2.5cm, height = 2.5cm]{./Figures/JBF/ImgNo5_Noise16_X_resid_JBF.eps}
		\end{minipage} 
		\begin{minipage}[b]{0.28\linewidth}
			\centering
			\includegraphics[width = 2.5cm, height = 2.5cm]{./Figures/JBF/ImgNo5_Noise24_X_resid_JBF.eps}
		\end{minipage} 
		\\
		% ------------------------------------------- 
		% GF
		\begin{minipage}[b]{0.1\linewidth}
			\centering
			{\footnotesize GF~\cite{he2013guided}}  
		\end{minipage}  
		\begin{minipage}[b]{0.28\linewidth}
			\centering
			\includegraphics[width = 2.5cm, height = 2.5cm]{./Figures/GF/ImgNo5_Noise8_X_GF.eps}
		\end{minipage} 
		\begin{minipage}[b]{0.28\linewidth}
			\centering
			\includegraphics[width = 2.5cm, height = 2.5cm]{./Figures/GF/ImgNo5_Noise16_X_GF.eps}
		\end{minipage} 
		\begin{minipage}[b]{0.28\linewidth}
			\centering
			\includegraphics[width = 2.5cm, height = 2.5cm]{./Figures/GF/ImgNo5_Noise24_X_GF.eps}
		\end{minipage} 
		\\
		% ------------------------------------------- 
		% GF
		\begin{minipage}[b]{0.1\linewidth}
			\centering
			{\footnotesize ErrMap GF~\cite{he2013guided}}  
		\end{minipage} 
		\begin{minipage}[b]{0.28\linewidth}
			\centering
			\includegraphics[width = 2.5cm, height = 2.5cm]{./Figures/GF/ImgNo5_Noise8_X_resid_GF.eps}
		\end{minipage} 
		\begin{minipage}[b]{0.28\linewidth}
			\centering
			\includegraphics[width = 2.5cm, height = 2.5cm]{./Figures/GF/ImgNo5_Noise16_X_resid_GF.eps}
		\end{minipage} 
		\begin{minipage}[b]{0.28\linewidth}
			\centering
			\includegraphics[width = 2.5cm, height = 2.5cm]{./Figures/GF/ImgNo5_Noise24_X_resid_GF.eps}
		\end{minipage} 
		\\
		% -------------------------------------------
		% SDF
		\begin{minipage}[b]{0.1\linewidth}
			\centering
			{\footnotesize SDF~\cite{ham2017robust}} %  
		\end{minipage} 
		\begin{minipage}[b]{0.28\linewidth}
			\centering
			\includegraphics[width = 2.5cm, height = 2.5cm]{./Figures/SDF/ImgNo5_Noise8_X_SDF.eps}
		\end{minipage} 
		\begin{minipage}[b]{0.28\linewidth}
			\centering
			\includegraphics[width = 2.5cm, height = 2.5cm]{./Figures/SDF/ImgNo5_Noise16_X_SDF.eps}
		\end{minipage}  
		\begin{minipage}[b]{0.28\linewidth}
			\centering
			\includegraphics[width = 2.5cm, height = 2.5cm]{./Figures/SDF/ImgNo5_Noise24_X_SDF.eps}
		\end{minipage} 
		\\
		% -------------------------------------------
		% SDF
		\begin{minipage}[b]{0.1\linewidth}
			\centering
			{\footnotesize ErrMap SDF~\cite{ham2017robust}} % 
		\end{minipage}  
		\begin{minipage}[b]{0.28\linewidth}
			\centering
			\includegraphics[width = 2.5cm, height = 2.5cm]{./Figures/SDF/ImgNo5_Noise8_X_resid_SDF.eps}
		\end{minipage} 
		\begin{minipage}[b]{0.28\linewidth}
			\centering
			\includegraphics[width = 2.5cm, height = 2.5cm]{./Figures/SDF/ImgNo5_Noise16_X_resid_SDF.eps}
		\end{minipage} 
		\begin{minipage}[b]{0.28\linewidth}
			\centering
			\includegraphics[width = 2.5cm, height = 2.5cm]{./Figures/SDF/ImgNo5_Noise24_X_resid_SDF.eps}
		\end{minipage} 
		\\
		% ------------------------------------------- 
		\begin{minipage}[b]{0.1\linewidth}
			\centering	% {\phantom{{\footnotesize XXX}}} 
		\end{minipage}
		\begin{minipage}[b]{0.28\linewidth}
			\centering	{\footnotesize $\sigma=8$}
		\end{minipage} 
		\begin{minipage}[b]{0.28\linewidth}
			\centering	{\footnotesize $\sigma=16$} 
		\end{minipage} 
		\begin{minipage}[b]{0.28\linewidth}
			\centering	{\footnotesize $\sigma=24$} 
		\end{minipage}
		\\
		%---------------------------------------------------
		% true images
		\begin{minipage}[b]{0.1\linewidth}
			\centering
			{\footnotesize Truth}  
		\end{minipage} 
		\begin{minipage}[b]{0.28\linewidth}
			\centering
			\includegraphics[width = 2.5cm, height = 2.5cm]{./Figures/GF/ImgNo5_Noise8_X_true.eps}
		\end{minipage} 
		\begin{minipage}[b]{0.28\linewidth}
			\centering
			\includegraphics[width = 2.5cm, height = 2.5cm]{./Figures/GF/ImgNo5_Noise16_X_true.eps}
		\end{minipage} 
		\begin{minipage}[b]{0.28\linewidth}
			\centering
			\includegraphics[width = 2.5cm, height = 2.5cm]{./Figures/GF/ImgNo5_Noise24_X_true.eps}
		\end{minipage} 
		\\
		% -------------------------------------------
		% JFSM
		\begin{minipage}[b]{0.1\linewidth}
			\centering
			{\footnotesize JFSM\cite{shen2015multispectral}}  
		\end{minipage}  
		\begin{minipage}[b]{0.28\linewidth}
			\centering
			\includegraphics[width = 2.5cm, height = 2.5cm]{./Figures/JFSM/ImgNo5_Noise8_X_JFSM.eps}
		\end{minipage}  
		\begin{minipage}[b]{0.28\linewidth}
			\centering
			\includegraphics[width = 2.5cm, height = 2.5cm]{./Figures/JFSM/ImgNo5_Noise16_X_JFSM.eps}
		\end{minipage} 
		\begin{minipage}[b]{0.28\linewidth}
			\centering
			\includegraphics[width = 2.5cm, height = 2.5cm]{./Figures/JFSM/ImgNo5_Noise24_X_JFSM.eps}
		\end{minipage} 
		\\
		% -------------------------------------------	
		% JFSM
		\begin{minipage}[b]{0.1\linewidth}
			\centering
			{\footnotesize ErrMap JFSM\cite{shen2015multispectral}}  
		\end{minipage} 
		\begin{minipage}[b]{0.28\linewidth}
			\centering
			\includegraphics[width = 2.5cm, height = 2.5cm]{./Figures/JFSM/ImgNo5_Noise8_X_resid_JFSM.eps}
		\end{minipage} 
		\begin{minipage}[b]{0.28\linewidth}
			\centering
			\includegraphics[width = 2.5cm, height = 2.5cm]{./Figures/JFSM/ImgNo5_Noise16_X_resid_JFSM.eps}
		\end{minipage} 
		\begin{minipage}[b]{0.28\linewidth}
			\centering
			\includegraphics[width = 2.5cm, height = 2.5cm]{./Figures/JFSM/ImgNo5_Noise24_X_resid_JFSM.eps}
		\end{minipage} 
		\\
		% -------------------------------------------
		% DJF
		\begin{minipage}[b]{0.1\linewidth}
			\centering
			{\footnotesize DJF~\cite{li2016deep}} %  
		\end{minipage} 
		\begin{minipage}[b]{0.28\linewidth}
			\centering
			\includegraphics[width = 2.5cm, height = 2.5cm]{./Figures/DJF/ImgNo5_Noise8_X_DJF.eps}
		\end{minipage} 
		\begin{minipage}[b]{0.28\linewidth}
			\centering
			\includegraphics[width = 2.5cm, height = 2.5cm]{./Figures/DJF/ImgNo5_Noise16_X_DJF.eps}
		\end{minipage} 
		\begin{minipage}[b]{0.28\linewidth}
			\centering
			\includegraphics[width = 2.5cm, height = 2.5cm]{./Figures/DJF/ImgNo5_Noise24_X_DJF.eps}
		\end{minipage} 
		\\
		% -------------------------------------------
		% DJF
		\begin{minipage}[b]{0.1\linewidth}
			\centering
			{\footnotesize ErrMap DJF~\cite{li2016deep}} %  
		\end{minipage}  
		\begin{minipage}[b]{0.28\linewidth}
			\centering
			\includegraphics[width = 2.5cm, height = 2.5cm]{./Figures/DJF/ImgNo5_Noise8_X_resid_DJF.eps}
		\end{minipage} 
		\begin{minipage}[b]{0.28\linewidth}
			\centering
			\includegraphics[width = 2.5cm, height = 2.5cm]{./Figures/DJF/ImgNo5_Noise16_X_resid_DJF.eps}
		\end{minipage} 
		\begin{minipage}[b]{0.28\linewidth}
			\centering
			\includegraphics[width = 2.5cm, height = 2.5cm]{./Figures/DJF/ImgNo5_Noise24_X_resid_DJF.eps}
		\end{minipage} 
		\\
		% -------------------------------------------
		%	% CDN with standard sparsity
		%	\begin{minipage}[b]{0.1\linewidth}
		%		\centering
		%		{\footnotesize Ours} %  
		%	\end{minipage} 
		%	\begin{minipage}[b]{0.28\linewidth}
		%		\centering
		%		\includegraphics[width = 2.5cm, height = 2.5cm]{./Figures/CDN/ImgNo5_Noise4_X_CDN.eps}
		%	\end{minipage} 
		%	\begin{minipage}[b]{0.28\linewidth}
		%		\centering
		%		\includegraphics[width = 2.5cm, height = 2.5cm]{./Figures/CDN/ImgNo5_Noise12_X_CDN.eps}
		%	\end{minipage} 
		%	\begin{minipage}[b]{0.28\linewidth}
		%		\centering
		%		\includegraphics[width = 2.5cm, height = 2.5cm]{./Figures/CDN/ImgNo5_Noise20_X_CDN.eps}
		%	\end{minipage} 
		%	\\
		% -------------------------------------------
		%	% CDN with standard sparsity
		%	\begin{minipage}[b]{0.1\linewidth}
		%		\centering
		%		{\footnotesize ErrMap Ours} %  
		%	\end{minipage} 
		%	\begin{minipage}[b]{0.28\linewidth}
		%		\centering
		%		\includegraphics[width = 2.5cm, height = 2.5cm]{./Figures/CDN/ImgNo5_Noise8_X_resid_CDN.eps}
		%	\end{minipage} 
		%	\begin{minipage}[b]{0.28\linewidth}
		%		\centering
		%		\includegraphics[width = 2.5cm, height = 2.5cm]{./Figures/CDN/ImgNo5_Noise16_X_resid_CDN.eps}
		%	\end{minipage} 
		%	\begin{minipage}[b]{0.28\linewidth}
		%		\centering
		%		\includegraphics[width = 2.5cm, height = 2.5cm]{./Figures/CDN/ImgNo5_Noise24_X_resid_CDN.eps}
		%	\end{minipage} 
		%	\\
		% -------------------------------------------
		% CDN with group sparsity
		\begin{minipage}[b]{0.1\linewidth}
			\centering
			{\footnotesize Ours+}  
		\end{minipage} 
		\begin{minipage}[b]{0.28\linewidth}
			\centering
			\includegraphics[width = 2.5cm, height = 2.5cm]{./Figures/CDN_GrpSp/ImgNo5_Noise8_X_CDN.eps}
		\end{minipage} 
		\begin{minipage}[b]{0.28\linewidth}
			\centering
			\includegraphics[width = 2.5cm, height = 2.5cm]{./Figures/CDN_GrpSp/ImgNo5_Noise16_X_CDN.eps}
		\end{minipage} 
		\begin{minipage}[b]{0.28\linewidth}
			\centering
			\includegraphics[width = 2.5cm, height = 2.5cm]{./Figures/CDN_GrpSp/ImgNo5_Noise24_X_CDN.eps}
		\end{minipage} 
		\\
		% -------------------------------------------
		% CDN with group sparsity
		\begin{minipage}[b]{0.1\linewidth}
			\centering
			{\footnotesize ErrMap Ours+}  
		\end{minipage} 
		\begin{minipage}[b]{0.28\linewidth}
			\centering
			\includegraphics[width = 2.5cm, height = 2.5cm]{./Figures/CDN_GrpSp/ImgNo5_Noise8_X_resid_CDN.eps}
		\end{minipage} 
		\begin{minipage}[b]{0.28\linewidth}
			\centering
			\includegraphics[width = 2.5cm, height = 2.5cm]{./Figures/CDN_GrpSp/ImgNo5_Noise16_X_resid_CDN.eps}
		\end{minipage} 
		\begin{minipage}[b]{0.28\linewidth}
			\centering
			\includegraphics[width = 2.5cm, height = 2.5cm]{./Figures/CDN_GrpSp/ImgNo5_Noise24_X_resid_CDN.eps}
		\end{minipage} 
		\\
		% ------------------------------------------- 
		\begin{minipage}[b]{0.1\linewidth}
			\centering	% {\phantom{{\footnotesize XXX}}} 
		\end{minipage}
		\begin{minipage}[b]{0.28\linewidth}
			\centering	{\footnotesize $\sigma=8$}
		\end{minipage} 
		\begin{minipage}[b]{0.28\linewidth}
			\centering	{\footnotesize $\sigma=16$} 
		\end{minipage} 
		\begin{minipage}[b]{0.28\linewidth}
			\centering	{\footnotesize $\sigma=24$} 
		\end{minipage}
		% -------------------------------------------	
	\end{multicols}	
	
	\vspace{-0.8cm}
	
	\begin{multicols}{1}  
		\begin{minipage}[b]{0.98\linewidth}
			{\footnotesize Colorbar}
			\includegraphics[width = 16.8cm, height=0.5cm]{./Figures/Colorbar64.eps}
		\end{minipage}
	\end{multicols}	
	
	\vspace{-0.6cm}
	
	\caption{Visual comparison on multimodal image denoising.}
	%	 Each row represents one approach and its denoising results corresponding to different noise levels.}
	\label{Fig:DenoisedIms_5}
\end{figure*}

%%================================================================================================

%% image No6 -- denoised images for only 3 noise levels
\begin{figure*}[th]
	\begin{multicols}{2}  
		\centering
		% ------------------------------------------- 
		% Noisy images
		\begin{minipage}[b]{0.1\linewidth}
			\centering
			{\footnotesize Input}  
		\end{minipage} 
		\begin{minipage}[b]{0.28\linewidth}
			\centering
			\includegraphics[width = 2.5cm, height = 2.5cm]{./Figures/GF/ImgNo6_Noise8_X_low.eps}
		\end{minipage} 
		\begin{minipage}[b]{0.28\linewidth}
			\centering
			\includegraphics[width = 2.5cm, height = 2.5cm]{./Figures/GF/ImgNo6_Noise16_X_low.eps}
		\end{minipage} 
		\begin{minipage}[b]{0.28\linewidth}
			\centering
			\includegraphics[width = 2.5cm, height = 2.5cm]{./Figures/GF/ImgNo6_Noise24_X_low.eps}
		\end{minipage} 
		\\
		% ------------------------------------------- 
		% JBF
		\begin{minipage}[b]{0.1\linewidth}
			\centering
			{\footnotesize JBF~\cite{kopf2007joint}} % 
		\end{minipage} 
		\begin{minipage}[b]{0.28\linewidth}
			\centering
			\includegraphics[width = 2.5cm, height = 2.5cm]{./Figures/JBF/ImgNo6_Noise8_X_JBF.eps}
		\end{minipage}  
		\begin{minipage}[b]{0.28\linewidth}
			\centering
			\includegraphics[width = 2.5cm, height = 2.5cm]{./Figures/JBF/ImgNo6_Noise16_X_JBF.eps}
		\end{minipage} 
		\begin{minipage}[b]{0.28\linewidth}
			\centering
			\includegraphics[width = 2.5cm, height = 2.5cm]{./Figures/JBF/ImgNo6_Noise24_X_JBF.eps}
		\end{minipage} 
		\\
		% ------------------------------------------- 
		% JBF
		\begin{minipage}[b]{0.1\linewidth}
			\centering
			{\footnotesize ErrMap JBF~\cite{kopf2007joint}} % 
		\end{minipage} 
		\begin{minipage}[b]{0.28\linewidth}
			\centering
			\includegraphics[width = 2.5cm, height = 2.5cm]{./Figures/JBF/ImgNo6_Noise8_X_resid_JBF.eps}
		\end{minipage} 
		\begin{minipage}[b]{0.28\linewidth}
			\centering
			\includegraphics[width = 2.5cm, height = 2.5cm]{./Figures/JBF/ImgNo6_Noise16_X_resid_JBF.eps}
		\end{minipage} 
		\begin{minipage}[b]{0.28\linewidth}
			\centering
			\includegraphics[width = 2.5cm, height = 2.5cm]{./Figures/JBF/ImgNo6_Noise24_X_resid_JBF.eps}
		\end{minipage} 
		\\
		% ------------------------------------------- 
		% GF
		\begin{minipage}[b]{0.1\linewidth}
			\centering
			{\footnotesize GF~\cite{he2013guided}}  
		\end{minipage}  
		\begin{minipage}[b]{0.28\linewidth}
			\centering
			\includegraphics[width = 2.5cm, height = 2.5cm]{./Figures/GF/ImgNo6_Noise8_X_GF.eps}
		\end{minipage} 
		\begin{minipage}[b]{0.28\linewidth}
			\centering
			\includegraphics[width = 2.5cm, height = 2.5cm]{./Figures/GF/ImgNo6_Noise16_X_GF.eps}
		\end{minipage} 
		\begin{minipage}[b]{0.28\linewidth}
			\centering
			\includegraphics[width = 2.5cm, height = 2.5cm]{./Figures/GF/ImgNo6_Noise24_X_GF.eps}
		\end{minipage} 
		\\
		% ------------------------------------------- 
		% GF
		\begin{minipage}[b]{0.1\linewidth}
			\centering
			{\footnotesize ErrMap GF~\cite{he2013guided}}  
		\end{minipage} 
		\begin{minipage}[b]{0.28\linewidth}
			\centering
			\includegraphics[width = 2.5cm, height = 2.5cm]{./Figures/GF/ImgNo6_Noise8_X_resid_GF.eps}
		\end{minipage} 
		\begin{minipage}[b]{0.28\linewidth}
			\centering
			\includegraphics[width = 2.5cm, height = 2.5cm]{./Figures/GF/ImgNo6_Noise16_X_resid_GF.eps}
		\end{minipage} 
		\begin{minipage}[b]{0.28\linewidth}
			\centering
			\includegraphics[width = 2.5cm, height = 2.5cm]{./Figures/GF/ImgNo6_Noise24_X_resid_GF.eps}
		\end{minipage} 
		\\
		% -------------------------------------------
		% SDF
		\begin{minipage}[b]{0.1\linewidth}
			\centering
			{\footnotesize SDF~\cite{ham2017robust}} %  
		\end{minipage} 
		\begin{minipage}[b]{0.28\linewidth}
			\centering
			\includegraphics[width = 2.5cm, height = 2.5cm]{./Figures/SDF/ImgNo6_Noise8_X_SDF.eps}
		\end{minipage} 
		\begin{minipage}[b]{0.28\linewidth}
			\centering
			\includegraphics[width = 2.5cm, height = 2.5cm]{./Figures/SDF/ImgNo6_Noise16_X_SDF.eps}
		\end{minipage}  
		\begin{minipage}[b]{0.28\linewidth}
			\centering
			\includegraphics[width = 2.5cm, height = 2.5cm]{./Figures/SDF/ImgNo6_Noise24_X_SDF.eps}
		\end{minipage} 
		\\
		% -------------------------------------------
		% SDF
		\begin{minipage}[b]{0.1\linewidth}
			\centering
			{\footnotesize ErrMap SDF~\cite{ham2017robust}} % 
		\end{minipage}  
		\begin{minipage}[b]{0.28\linewidth}
			\centering
			\includegraphics[width = 2.5cm, height = 2.5cm]{./Figures/SDF/ImgNo6_Noise8_X_resid_SDF.eps}
		\end{minipage} 
		\begin{minipage}[b]{0.28\linewidth}
			\centering
			\includegraphics[width = 2.5cm, height = 2.5cm]{./Figures/SDF/ImgNo6_Noise16_X_resid_SDF.eps}
		\end{minipage} 
		\begin{minipage}[b]{0.28\linewidth}
			\centering
			\includegraphics[width = 2.5cm, height = 2.5cm]{./Figures/SDF/ImgNo6_Noise24_X_resid_SDF.eps}
		\end{minipage} 
		\\
		% ------------------------------------------- 
		\begin{minipage}[b]{0.1\linewidth}
			\centering	% {\phantom{{\footnotesize XXX}}} 
		\end{minipage}
		\begin{minipage}[b]{0.28\linewidth}
			\centering	{\footnotesize $\sigma=8$}
		\end{minipage} 
		\begin{minipage}[b]{0.28\linewidth}
			\centering	{\footnotesize $\sigma=16$} 
		\end{minipage} 
		\begin{minipage}[b]{0.28\linewidth}
			\centering	{\footnotesize $\sigma=24$} 
		\end{minipage}
		\\
		%---------------------------------------------------
		% true images
		\begin{minipage}[b]{0.1\linewidth}
			\centering
			{\footnotesize Truth}  
		\end{minipage} 
		\begin{minipage}[b]{0.28\linewidth}
			\centering
			\includegraphics[width = 2.5cm, height = 2.5cm]{./Figures/GF/ImgNo6_Noise8_X_true.eps}
		\end{minipage} 
		\begin{minipage}[b]{0.28\linewidth}
			\centering
			\includegraphics[width = 2.5cm, height = 2.5cm]{./Figures/GF/ImgNo6_Noise16_X_true.eps}
		\end{minipage} 
		\begin{minipage}[b]{0.28\linewidth}
			\centering
			\includegraphics[width = 2.5cm, height = 2.5cm]{./Figures/GF/ImgNo6_Noise24_X_true.eps}
		\end{minipage} 
		\\
		% -------------------------------------------
		% JFSM
		\begin{minipage}[b]{0.1\linewidth}
			\centering
			{\footnotesize JFSM\cite{shen2015multispectral}}  
		\end{minipage}  
		\begin{minipage}[b]{0.28\linewidth}
			\centering
			\includegraphics[width = 2.5cm, height = 2.5cm]{./Figures/JFSM/ImgNo6_Noise8_X_JFSM.eps}
		\end{minipage}  
		\begin{minipage}[b]{0.28\linewidth}
			\centering
			\includegraphics[width = 2.5cm, height = 2.5cm]{./Figures/JFSM/ImgNo6_Noise16_X_JFSM.eps}
		\end{minipage} 
		\begin{minipage}[b]{0.28\linewidth}
			\centering
			\includegraphics[width = 2.5cm, height = 2.5cm]{./Figures/JFSM/ImgNo6_Noise24_X_JFSM.eps}
		\end{minipage} 
		\\
		% -------------------------------------------	
		% JFSM
		\begin{minipage}[b]{0.1\linewidth}
			\centering
			{\footnotesize ErrMap JFSM\cite{shen2015multispectral}}  
		\end{minipage} 
		\begin{minipage}[b]{0.28\linewidth}
			\centering
			\includegraphics[width = 2.5cm, height = 2.5cm]{./Figures/JFSM/ImgNo6_Noise8_X_resid_JFSM.eps}
		\end{minipage} 
		\begin{minipage}[b]{0.28\linewidth}
			\centering
			\includegraphics[width = 2.5cm, height = 2.5cm]{./Figures/JFSM/ImgNo6_Noise16_X_resid_JFSM.eps}
		\end{minipage} 
		\begin{minipage}[b]{0.28\linewidth}
			\centering
			\includegraphics[width = 2.5cm, height = 2.5cm]{./Figures/JFSM/ImgNo6_Noise24_X_resid_JFSM.eps}
		\end{minipage} 
		\\
		% -------------------------------------------
		% DJF
		\begin{minipage}[b]{0.1\linewidth}
			\centering
			{\footnotesize DJF~\cite{li2016deep}} %  
		\end{minipage} 
		\begin{minipage}[b]{0.28\linewidth}
			\centering
			\includegraphics[width = 2.5cm, height = 2.5cm]{./Figures/DJF/ImgNo6_Noise8_X_DJF.eps}
		\end{minipage} 
		\begin{minipage}[b]{0.28\linewidth}
			\centering
			\includegraphics[width = 2.5cm, height = 2.5cm]{./Figures/DJF/ImgNo6_Noise16_X_DJF.eps}
		\end{minipage} 
		\begin{minipage}[b]{0.28\linewidth}
			\centering
			\includegraphics[width = 2.5cm, height = 2.5cm]{./Figures/DJF/ImgNo6_Noise24_X_DJF.eps}
		\end{minipage} 
		\\
		% -------------------------------------------
		% DJF
		\begin{minipage}[b]{0.1\linewidth}
			\centering
			{\footnotesize ErrMap DJF~\cite{li2016deep}} %  
		\end{minipage}  
		\begin{minipage}[b]{0.28\linewidth}
			\centering
			\includegraphics[width = 2.5cm, height = 2.5cm]{./Figures/DJF/ImgNo6_Noise8_X_resid_DJF.eps}
		\end{minipage} 
		\begin{minipage}[b]{0.28\linewidth}
			\centering
			\includegraphics[width = 2.5cm, height = 2.5cm]{./Figures/DJF/ImgNo6_Noise16_X_resid_DJF.eps}
		\end{minipage} 
		\begin{minipage}[b]{0.28\linewidth}
			\centering
			\includegraphics[width = 2.5cm, height = 2.5cm]{./Figures/DJF/ImgNo6_Noise24_X_resid_DJF.eps}
		\end{minipage} 
		\\
		% -------------------------------------------
		%	% CDN with standard sparsity
		%	\begin{minipage}[b]{0.1\linewidth}
		%		\centering
		%		{\footnotesize Ours} %  
		%	\end{minipage} 
		%	\begin{minipage}[b]{0.28\linewidth}
		%		\centering
		%		\includegraphics[width = 2.5cm, height = 2.5cm]{./Figures/CDN/ImgNo6_Noise4_X_CDN.eps}
		%	\end{minipage} 
		%	\begin{minipage}[b]{0.28\linewidth}
		%		\centering
		%		\includegraphics[width = 2.5cm, height = 2.5cm]{./Figures/CDN/ImgNo6_Noise12_X_CDN.eps}
		%	\end{minipage} 
		%	\begin{minipage}[b]{0.28\linewidth}
		%		\centering
		%		\includegraphics[width = 2.5cm, height = 2.5cm]{./Figures/CDN/ImgNo6_Noise20_X_CDN.eps}
		%	\end{minipage} 
		%	\\
		% -------------------------------------------
		%	% CDN with standard sparsity
		%	\begin{minipage}[b]{0.1\linewidth}
		%		\centering
		%		{\footnotesize ErrMap Ours} %  
		%	\end{minipage} 
		%	\begin{minipage}[b]{0.28\linewidth}
		%		\centering
		%		\includegraphics[width = 2.5cm, height = 2.5cm]{./Figures/CDN/ImgNo6_Noise8_X_resid_CDN.eps}
		%	\end{minipage} 
		%	\begin{minipage}[b]{0.28\linewidth}
		%		\centering
		%		\includegraphics[width = 2.5cm, height = 2.5cm]{./Figures/CDN/ImgNo6_Noise16_X_resid_CDN.eps}
		%	\end{minipage} 
		%	\begin{minipage}[b]{0.28\linewidth}
		%		\centering
		%		\includegraphics[width = 2.5cm, height = 2.5cm]{./Figures/CDN/ImgNo6_Noise24_X_resid_CDN.eps}
		%	\end{minipage} 
		%	\\
		% -------------------------------------------
		% CDN with group sparsity
		\begin{minipage}[b]{0.1\linewidth}
			\centering
			{\footnotesize Ours+}  
		\end{minipage} 
		\begin{minipage}[b]{0.28\linewidth}
			\centering
			\includegraphics[width = 2.5cm, height = 2.5cm]{./Figures/CDN_GrpSp/ImgNo6_Noise8_X_CDN.eps}
		\end{minipage} 
		\begin{minipage}[b]{0.28\linewidth}
			\centering
			\includegraphics[width = 2.5cm, height = 2.5cm]{./Figures/CDN_GrpSp/ImgNo6_Noise16_X_CDN.eps}
		\end{minipage} 
		\begin{minipage}[b]{0.28\linewidth}
			\centering
			\includegraphics[width = 2.5cm, height = 2.5cm]{./Figures/CDN_GrpSp/ImgNo6_Noise24_X_CDN.eps}
		\end{minipage} 
		\\
		% -------------------------------------------
		% CDN with group sparsity
		\begin{minipage}[b]{0.1\linewidth}
			\centering
			{\footnotesize ErrMap Ours+}  
		\end{minipage} 
		\begin{minipage}[b]{0.28\linewidth}
			\centering
			\includegraphics[width = 2.5cm, height = 2.5cm]{./Figures/CDN_GrpSp/ImgNo6_Noise8_X_resid_CDN.eps}
		\end{minipage} 
		\begin{minipage}[b]{0.28\linewidth}
			\centering
			\includegraphics[width = 2.5cm, height = 2.5cm]{./Figures/CDN_GrpSp/ImgNo6_Noise16_X_resid_CDN.eps}
		\end{minipage} 
		\begin{minipage}[b]{0.28\linewidth}
			\centering
			\includegraphics[width = 2.5cm, height = 2.5cm]{./Figures/CDN_GrpSp/ImgNo6_Noise24_X_resid_CDN.eps}
		\end{minipage} 
		\\
		% ------------------------------------------- 
		\begin{minipage}[b]{0.1\linewidth}
			\centering	% {\phantom{{\footnotesize XXX}}} 
		\end{minipage}
		\begin{minipage}[b]{0.28\linewidth}
			\centering	{\footnotesize $\sigma=8$}
		\end{minipage} 
		\begin{minipage}[b]{0.28\linewidth}
			\centering	{\footnotesize $\sigma=16$} 
		\end{minipage} 
		\begin{minipage}[b]{0.28\linewidth}
			\centering	{\footnotesize $\sigma=24$} 
		\end{minipage}
		% -------------------------------------------	
	\end{multicols}	
	
	\vspace{-0.8cm}
	
	\begin{multicols}{1}  
		\begin{minipage}[b]{0.98\linewidth}
			{\footnotesize Colorbar}
			\includegraphics[width = 16.8cm, height=0.5cm]{./Figures/Colorbar64.eps}
		\end{minipage}
	\end{multicols}	
	
	\vspace{-0.6cm}
	
	\caption{Visual comparison on multimodal image denoising.}
	%	 Each row represents one approach and its denoising results corresponding to different noise levels.}
	\label{Fig:DenoisedIms_6}
\end{figure*}

%%=====================================================================================

%% image No7 -- denoised images for only 3 noise levels
\begin{figure*}[th]
	\begin{multicols}{2}  
		\centering
		% ------------------------------------------- 
		% Noisy images
		\begin{minipage}[b]{0.1\linewidth}
			\centering
			{\footnotesize Input}  
		\end{minipage} 
		\begin{minipage}[b]{0.28\linewidth}
			\centering
			\includegraphics[width = 2.5cm, height = 2.5cm]{./Figures/GF/ImgNo7_Noise8_X_low.eps}
		\end{minipage} 
		\begin{minipage}[b]{0.28\linewidth}
			\centering
			\includegraphics[width = 2.5cm, height = 2.5cm]{./Figures/GF/ImgNo7_Noise16_X_low.eps}
		\end{minipage} 
		\begin{minipage}[b]{0.28\linewidth}
			\centering
			\includegraphics[width = 2.5cm, height = 2.5cm]{./Figures/GF/ImgNo7_Noise24_X_low.eps}
		\end{minipage} 
		\\
		% ------------------------------------------- 
		% JBF
		\begin{minipage}[b]{0.1\linewidth}
			\centering
			{\footnotesize JBF~\cite{kopf2007joint}} % 
		\end{minipage} 
		\begin{minipage}[b]{0.28\linewidth}
			\centering
			\includegraphics[width = 2.5cm, height = 2.5cm]{./Figures/JBF/ImgNo7_Noise8_X_JBF.eps}
		\end{minipage}  
		\begin{minipage}[b]{0.28\linewidth}
			\centering
			\includegraphics[width = 2.5cm, height = 2.5cm]{./Figures/JBF/ImgNo7_Noise16_X_JBF.eps}
		\end{minipage} 
		\begin{minipage}[b]{0.28\linewidth}
			\centering
			\includegraphics[width = 2.5cm, height = 2.5cm]{./Figures/JBF/ImgNo7_Noise24_X_JBF.eps}
		\end{minipage} 
		\\
		% ------------------------------------------- 
		% JBF
		\begin{minipage}[b]{0.1\linewidth}
			\centering
			{\footnotesize ErrMap JBF~\cite{kopf2007joint}} % 
		\end{minipage} 
		\begin{minipage}[b]{0.28\linewidth}
			\centering
			\includegraphics[width = 2.5cm, height = 2.5cm]{./Figures/JBF/ImgNo7_Noise8_X_resid_JBF.eps}
		\end{minipage} 
		\begin{minipage}[b]{0.28\linewidth}
			\centering
			\includegraphics[width = 2.5cm, height = 2.5cm]{./Figures/JBF/ImgNo7_Noise16_X_resid_JBF.eps}
		\end{minipage} 
		\begin{minipage}[b]{0.28\linewidth}
			\centering
			\includegraphics[width = 2.5cm, height = 2.5cm]{./Figures/JBF/ImgNo7_Noise24_X_resid_JBF.eps}
		\end{minipage} 
		\\
		% ------------------------------------------- 
		% GF
		\begin{minipage}[b]{0.1\linewidth}
			\centering
			{\footnotesize GF~\cite{he2013guided}}  
		\end{minipage}  
		\begin{minipage}[b]{0.28\linewidth}
			\centering
			\includegraphics[width = 2.5cm, height = 2.5cm]{./Figures/GF/ImgNo7_Noise8_X_GF.eps}
		\end{minipage} 
		\begin{minipage}[b]{0.28\linewidth}
			\centering
			\includegraphics[width = 2.5cm, height = 2.5cm]{./Figures/GF/ImgNo7_Noise16_X_GF.eps}
		\end{minipage} 
		\begin{minipage}[b]{0.28\linewidth}
			\centering
			\includegraphics[width = 2.5cm, height = 2.5cm]{./Figures/GF/ImgNo7_Noise24_X_GF.eps}
		\end{minipage} 
		\\
		% ------------------------------------------- 
		% GF
		\begin{minipage}[b]{0.1\linewidth}
			\centering
			{\footnotesize ErrMap GF~\cite{he2013guided}}  
		\end{minipage} 
		\begin{minipage}[b]{0.28\linewidth}
			\centering
			\includegraphics[width = 2.5cm, height = 2.5cm]{./Figures/GF/ImgNo7_Noise8_X_resid_GF.eps}
		\end{minipage} 
		\begin{minipage}[b]{0.28\linewidth}
			\centering
			\includegraphics[width = 2.5cm, height = 2.5cm]{./Figures/GF/ImgNo7_Noise16_X_resid_GF.eps}
		\end{minipage} 
		\begin{minipage}[b]{0.28\linewidth}
			\centering
			\includegraphics[width = 2.5cm, height = 2.5cm]{./Figures/GF/ImgNo7_Noise24_X_resid_GF.eps}
		\end{minipage} 
		\\
		% -------------------------------------------
		% SDF
		\begin{minipage}[b]{0.1\linewidth}
			\centering
			{\footnotesize SDF~\cite{ham2017robust}} %  
		\end{minipage} 
		\begin{minipage}[b]{0.28\linewidth}
			\centering
			\includegraphics[width = 2.5cm, height = 2.5cm]{./Figures/SDF/ImgNo7_Noise8_X_SDF.eps}
		\end{minipage} 
		\begin{minipage}[b]{0.28\linewidth}
			\centering
			\includegraphics[width = 2.5cm, height = 2.5cm]{./Figures/SDF/ImgNo7_Noise16_X_SDF.eps}
		\end{minipage}  
		\begin{minipage}[b]{0.28\linewidth}
			\centering
			\includegraphics[width = 2.5cm, height = 2.5cm]{./Figures/SDF/ImgNo7_Noise24_X_SDF.eps}
		\end{minipage} 
		\\
		% -------------------------------------------
		% SDF
		\begin{minipage}[b]{0.1\linewidth}
			\centering
			{\footnotesize ErrMap SDF~\cite{ham2017robust}} % 
		\end{minipage}  
		\begin{minipage}[b]{0.28\linewidth}
			\centering
			\includegraphics[width = 2.5cm, height = 2.5cm]{./Figures/SDF/ImgNo7_Noise8_X_resid_SDF.eps}
		\end{minipage} 
		\begin{minipage}[b]{0.28\linewidth}
			\centering
			\includegraphics[width = 2.5cm, height = 2.5cm]{./Figures/SDF/ImgNo7_Noise16_X_resid_SDF.eps}
		\end{minipage} 
		\begin{minipage}[b]{0.28\linewidth}
			\centering
			\includegraphics[width = 2.5cm, height = 2.5cm]{./Figures/SDF/ImgNo7_Noise24_X_resid_SDF.eps}
		\end{minipage} 
		\\
		% ------------------------------------------- 
		\begin{minipage}[b]{0.1\linewidth}
			\centering	% {\phantom{{\footnotesize XXX}}} 
		\end{minipage}
		\begin{minipage}[b]{0.28\linewidth}
			\centering	{\footnotesize $\sigma=8$}
		\end{minipage} 
		\begin{minipage}[b]{0.28\linewidth}
			\centering	{\footnotesize $\sigma=16$} 
		\end{minipage} 
		\begin{minipage}[b]{0.28\linewidth}
			\centering	{\footnotesize $\sigma=24$} 
		\end{minipage}
		\\
		%---------------------------------------------------
		% true images
		\begin{minipage}[b]{0.1\linewidth}
			\centering
			{\footnotesize Truth}  
		\end{minipage} 
		\begin{minipage}[b]{0.28\linewidth}
			\centering
			\includegraphics[width = 2.5cm, height = 2.5cm]{./Figures/GF/ImgNo7_Noise8_X_true.eps}
		\end{minipage} 
		\begin{minipage}[b]{0.28\linewidth}
			\centering
			\includegraphics[width = 2.5cm, height = 2.5cm]{./Figures/GF/ImgNo7_Noise16_X_true.eps}
		\end{minipage} 
		\begin{minipage}[b]{0.28\linewidth}
			\centering
			\includegraphics[width = 2.5cm, height = 2.5cm]{./Figures/GF/ImgNo7_Noise24_X_true.eps}
		\end{minipage} 
		\\
		% -------------------------------------------
		% JFSM
		\begin{minipage}[b]{0.1\linewidth}
			\centering
			{\footnotesize JFSM\cite{shen2015multispectral}}  
		\end{minipage}  
		\begin{minipage}[b]{0.28\linewidth}
			\centering
			\includegraphics[width = 2.5cm, height = 2.5cm]{./Figures/JFSM/ImgNo7_Noise8_X_JFSM.eps}
		\end{minipage}  
		\begin{minipage}[b]{0.28\linewidth}
			\centering
			\includegraphics[width = 2.5cm, height = 2.5cm]{./Figures/JFSM/ImgNo7_Noise16_X_JFSM.eps}
		\end{minipage} 
		\begin{minipage}[b]{0.28\linewidth}
			\centering
			\includegraphics[width = 2.5cm, height = 2.5cm]{./Figures/JFSM/ImgNo7_Noise24_X_JFSM.eps}
		\end{minipage} 
		\\
		% -------------------------------------------	
		% JFSM
		\begin{minipage}[b]{0.1\linewidth}
			\centering
			{\footnotesize ErrMap JFSM\cite{shen2015multispectral}}  
		\end{minipage} 
		\begin{minipage}[b]{0.28\linewidth}
			\centering
			\includegraphics[width = 2.5cm, height = 2.5cm]{./Figures/JFSM/ImgNo7_Noise8_X_resid_JFSM.eps}
		\end{minipage} 
		\begin{minipage}[b]{0.28\linewidth}
			\centering
			\includegraphics[width = 2.5cm, height = 2.5cm]{./Figures/JFSM/ImgNo7_Noise16_X_resid_JFSM.eps}
		\end{minipage} 
		\begin{minipage}[b]{0.28\linewidth}
			\centering
			\includegraphics[width = 2.5cm, height = 2.5cm]{./Figures/JFSM/ImgNo7_Noise24_X_resid_JFSM.eps}
		\end{minipage} 
		\\
		% -------------------------------------------
		% DJF
		\begin{minipage}[b]{0.1\linewidth}
			\centering
			{\footnotesize DJF~\cite{li2016deep}} %  
		\end{minipage} 
		\begin{minipage}[b]{0.28\linewidth}
			\centering
			\includegraphics[width = 2.5cm, height = 2.5cm]{./Figures/DJF/ImgNo7_Noise8_X_DJF.eps}
		\end{minipage} 
		\begin{minipage}[b]{0.28\linewidth}
			\centering
			\includegraphics[width = 2.5cm, height = 2.5cm]{./Figures/DJF/ImgNo7_Noise16_X_DJF.eps}
		\end{minipage} 
		\begin{minipage}[b]{0.28\linewidth}
			\centering
			\includegraphics[width = 2.5cm, height = 2.5cm]{./Figures/DJF/ImgNo7_Noise24_X_DJF.eps}
		\end{minipage} 
		\\
		% -------------------------------------------
		% DJF
		\begin{minipage}[b]{0.1\linewidth}
			\centering
			{\footnotesize ErrMap DJF~\cite{li2016deep}} %  
		\end{minipage}  
		\begin{minipage}[b]{0.28\linewidth}
			\centering
			\includegraphics[width = 2.5cm, height = 2.5cm]{./Figures/DJF/ImgNo7_Noise8_X_resid_DJF.eps}
		\end{minipage} 
		\begin{minipage}[b]{0.28\linewidth}
			\centering
			\includegraphics[width = 2.5cm, height = 2.5cm]{./Figures/DJF/ImgNo7_Noise16_X_resid_DJF.eps}
		\end{minipage} 
		\begin{minipage}[b]{0.28\linewidth}
			\centering
			\includegraphics[width = 2.5cm, height = 2.5cm]{./Figures/DJF/ImgNo7_Noise24_X_resid_DJF.eps}
		\end{minipage} 
		\\
		% -------------------------------------------
		%	% CDN with standard sparsity
		%	\begin{minipage}[b]{0.1\linewidth}
		%		\centering
		%		{\footnotesize Ours} %  
		%	\end{minipage} 
		%	\begin{minipage}[b]{0.28\linewidth}
		%		\centering
		%		\includegraphics[width = 2.5cm, height = 2.5cm]{./Figures/CDN/ImgNo7_Noise4_X_CDN.eps}
		%	\end{minipage} 
		%	\begin{minipage}[b]{0.28\linewidth}
		%		\centering
		%		\includegraphics[width = 2.5cm, height = 2.5cm]{./Figures/CDN/ImgNo7_Noise12_X_CDN.eps}
		%	\end{minipage} 
		%	\begin{minipage}[b]{0.28\linewidth}
		%		\centering
		%		\includegraphics[width = 2.5cm, height = 2.5cm]{./Figures/CDN/ImgNo7_Noise20_X_CDN.eps}
		%	\end{minipage} 
		%	\\
		% -------------------------------------------
		%	% CDN with standard sparsity
		%	\begin{minipage}[b]{0.1\linewidth}
		%		\centering
		%		{\footnotesize ErrMap Ours} %  
		%	\end{minipage} 
		%	\begin{minipage}[b]{0.28\linewidth}
		%		\centering
		%		\includegraphics[width = 2.5cm, height = 2.5cm]{./Figures/CDN/ImgNo7_Noise8_X_resid_CDN.eps}
		%	\end{minipage} 
		%	\begin{minipage}[b]{0.28\linewidth}
		%		\centering
		%		\includegraphics[width = 2.5cm, height = 2.5cm]{./Figures/CDN/ImgNo7_Noise16_X_resid_CDN.eps}
		%	\end{minipage} 
		%	\begin{minipage}[b]{0.28\linewidth}
		%		\centering
		%		\includegraphics[width = 2.5cm, height = 2.5cm]{./Figures/CDN/ImgNo7_Noise24_X_resid_CDN.eps}
		%	\end{minipage} 
		%	\\
		% -------------------------------------------
		% CDN with group sparsity
		\begin{minipage}[b]{0.1\linewidth}
			\centering
			{\footnotesize Ours+}  
		\end{minipage} 
		\begin{minipage}[b]{0.28\linewidth}
			\centering
			\includegraphics[width = 2.5cm, height = 2.5cm]{./Figures/CDN_GrpSp/ImgNo7_Noise8_X_CDN.eps}
		\end{minipage} 
		\begin{minipage}[b]{0.28\linewidth}
			\centering
			\includegraphics[width = 2.5cm, height = 2.5cm]{./Figures/CDN_GrpSp/ImgNo7_Noise16_X_CDN.eps}
		\end{minipage} 
		\begin{minipage}[b]{0.28\linewidth}
			\centering
			\includegraphics[width = 2.5cm, height = 2.5cm]{./Figures/CDN_GrpSp/ImgNo7_Noise24_X_CDN.eps}
		\end{minipage} 
		\\
		% -------------------------------------------
		% CDN with group sparsity
		\begin{minipage}[b]{0.1\linewidth}
			\centering
			{\footnotesize ErrMap Ours+}  
		\end{minipage} 
		\begin{minipage}[b]{0.28\linewidth}
			\centering
			\includegraphics[width = 2.5cm, height = 2.5cm]{./Figures/CDN_GrpSp/ImgNo7_Noise8_X_resid_CDN.eps}
		\end{minipage} 
		\begin{minipage}[b]{0.28\linewidth}
			\centering
			\includegraphics[width = 2.5cm, height = 2.5cm]{./Figures/CDN_GrpSp/ImgNo7_Noise16_X_resid_CDN.eps}
		\end{minipage} 
		\begin{minipage}[b]{0.28\linewidth}
			\centering
			\includegraphics[width = 2.5cm, height = 2.5cm]{./Figures/CDN_GrpSp/ImgNo7_Noise24_X_resid_CDN.eps}
		\end{minipage} 
		\\
		% ------------------------------------------- 
		\begin{minipage}[b]{0.1\linewidth}
			\centering	% {\phantom{{\footnotesize XXX}}} 
		\end{minipage}
		\begin{minipage}[b]{0.28\linewidth}
			\centering	{\footnotesize $\sigma=8$}
		\end{minipage} 
		\begin{minipage}[b]{0.28\linewidth}
			\centering	{\footnotesize $\sigma=16$} 
		\end{minipage} 
		\begin{minipage}[b]{0.28\linewidth}
			\centering	{\footnotesize $\sigma=24$} 
		\end{minipage}
		% -------------------------------------------	
	\end{multicols}	
	
	\vspace{-0.8cm}
	
	\begin{multicols}{1}  
		\begin{minipage}[b]{0.98\linewidth}
			{\footnotesize Colorbar}
			\includegraphics[width = 16.8cm, height=0.5cm]{./Figures/Colorbar64.eps}
		\end{minipage}
	\end{multicols}	
	
	\vspace{-0.6cm}
	
	\caption{Visual comparison on multimodal image denoising.}
	%	 Each row represents one approach and its denoising results corresponding to different noise levels.}
	\label{Fig:DenoisedIms_7}
\end{figure*}

%%========================================================================================

%% image No8 -- denoised images for only 3 noise levels
\begin{figure*}[th]
	\begin{multicols}{2}  
		\centering
		% ------------------------------------------- 
		% Noisy images
		\begin{minipage}[b]{0.1\linewidth}
			\centering
			{\footnotesize Input}  
		\end{minipage} 
		\begin{minipage}[b]{0.28\linewidth}
			\centering
			\includegraphics[width = 2.5cm, height = 2.5cm]{./Figures/GF/ImgNo8_Noise8_X_low.eps}
		\end{minipage} 
		\begin{minipage}[b]{0.28\linewidth}
			\centering
			\includegraphics[width = 2.5cm, height = 2.5cm]{./Figures/GF/ImgNo8_Noise16_X_low.eps}
		\end{minipage} 
		\begin{minipage}[b]{0.28\linewidth}
			\centering
			\includegraphics[width = 2.5cm, height = 2.5cm]{./Figures/GF/ImgNo8_Noise24_X_low.eps}
		\end{minipage} 
		\\
		% ------------------------------------------- 
		% JBF
		\begin{minipage}[b]{0.1\linewidth}
			\centering
			{\footnotesize JBF~\cite{kopf2007joint}} % 
		\end{minipage} 
		\begin{minipage}[b]{0.28\linewidth}
			\centering
			\includegraphics[width = 2.5cm, height = 2.5cm]{./Figures/JBF/ImgNo8_Noise8_X_JBF.eps}
		\end{minipage}  
		\begin{minipage}[b]{0.28\linewidth}
			\centering
			\includegraphics[width = 2.5cm, height = 2.5cm]{./Figures/JBF/ImgNo8_Noise16_X_JBF.eps}
		\end{minipage} 
		\begin{minipage}[b]{0.28\linewidth}
			\centering
			\includegraphics[width = 2.5cm, height = 2.5cm]{./Figures/JBF/ImgNo8_Noise24_X_JBF.eps}
		\end{minipage} 
		\\
		% ------------------------------------------- 
		% JBF
		\begin{minipage}[b]{0.1\linewidth}
			\centering
			{\footnotesize ErrMap JBF~\cite{kopf2007joint}} % 
		\end{minipage} 
		\begin{minipage}[b]{0.28\linewidth}
			\centering
			\includegraphics[width = 2.5cm, height = 2.5cm]{./Figures/JBF/ImgNo8_Noise8_X_resid_JBF.eps}
		\end{minipage} 
		\begin{minipage}[b]{0.28\linewidth}
			\centering
			\includegraphics[width = 2.5cm, height = 2.5cm]{./Figures/JBF/ImgNo8_Noise16_X_resid_JBF.eps}
		\end{minipage} 
		\begin{minipage}[b]{0.28\linewidth}
			\centering
			\includegraphics[width = 2.5cm, height = 2.5cm]{./Figures/JBF/ImgNo8_Noise24_X_resid_JBF.eps}
		\end{minipage} 
		\\
		% ------------------------------------------- 
		% GF
		\begin{minipage}[b]{0.1\linewidth}
			\centering
			{\footnotesize GF~\cite{he2013guided}}  
		\end{minipage}  
		\begin{minipage}[b]{0.28\linewidth}
			\centering
			\includegraphics[width = 2.5cm, height = 2.5cm]{./Figures/GF/ImgNo8_Noise8_X_GF.eps}
		\end{minipage} 
		\begin{minipage}[b]{0.28\linewidth}
			\centering
			\includegraphics[width = 2.5cm, height = 2.5cm]{./Figures/GF/ImgNo8_Noise16_X_GF.eps}
		\end{minipage} 
		\begin{minipage}[b]{0.28\linewidth}
			\centering
			\includegraphics[width = 2.5cm, height = 2.5cm]{./Figures/GF/ImgNo8_Noise24_X_GF.eps}
		\end{minipage} 
		\\
		% ------------------------------------------- 
		% GF
		\begin{minipage}[b]{0.1\linewidth}
			\centering
			{\footnotesize ErrMap GF~\cite{he2013guided}}  
		\end{minipage} 
		\begin{minipage}[b]{0.28\linewidth}
			\centering
			\includegraphics[width = 2.5cm, height = 2.5cm]{./Figures/GF/ImgNo8_Noise8_X_resid_GF.eps}
		\end{minipage} 
		\begin{minipage}[b]{0.28\linewidth}
			\centering
			\includegraphics[width = 2.5cm, height = 2.5cm]{./Figures/GF/ImgNo8_Noise16_X_resid_GF.eps}
		\end{minipage} 
		\begin{minipage}[b]{0.28\linewidth}
			\centering
			\includegraphics[width = 2.5cm, height = 2.5cm]{./Figures/GF/ImgNo8_Noise24_X_resid_GF.eps}
		\end{minipage} 
		\\
		% -------------------------------------------
		% SDF
		\begin{minipage}[b]{0.1\linewidth}
			\centering
			{\footnotesize SDF~\cite{ham2017robust}} %  
		\end{minipage} 
		\begin{minipage}[b]{0.28\linewidth}
			\centering
			\includegraphics[width = 2.5cm, height = 2.5cm]{./Figures/SDF/ImgNo8_Noise8_X_SDF.eps}
		\end{minipage} 
		\begin{minipage}[b]{0.28\linewidth}
			\centering
			\includegraphics[width = 2.5cm, height = 2.5cm]{./Figures/SDF/ImgNo8_Noise16_X_SDF.eps}
		\end{minipage}  
		\begin{minipage}[b]{0.28\linewidth}
			\centering
			\includegraphics[width = 2.5cm, height = 2.5cm]{./Figures/SDF/ImgNo8_Noise24_X_SDF.eps}
		\end{minipage} 
		\\
		% -------------------------------------------
		% SDF
		\begin{minipage}[b]{0.1\linewidth}
			\centering
			{\footnotesize ErrMap SDF~\cite{ham2017robust}} % 
		\end{minipage}  
		\begin{minipage}[b]{0.28\linewidth}
			\centering
			\includegraphics[width = 2.5cm, height = 2.5cm]{./Figures/SDF/ImgNo8_Noise8_X_resid_SDF.eps}
		\end{minipage} 
		\begin{minipage}[b]{0.28\linewidth}
			\centering
			\includegraphics[width = 2.5cm, height = 2.5cm]{./Figures/SDF/ImgNo8_Noise16_X_resid_SDF.eps}
		\end{minipage} 
		\begin{minipage}[b]{0.28\linewidth}
			\centering
			\includegraphics[width = 2.5cm, height = 2.5cm]{./Figures/SDF/ImgNo8_Noise24_X_resid_SDF.eps}
		\end{minipage} 
		\\
		% ------------------------------------------- 
		\begin{minipage}[b]{0.1\linewidth}
			\centering	% {\phantom{{\footnotesize XXX}}} 
		\end{minipage}
		\begin{minipage}[b]{0.28\linewidth}
			\centering	{\footnotesize $\sigma=8$}
		\end{minipage} 
		\begin{minipage}[b]{0.28\linewidth}
			\centering	{\footnotesize $\sigma=16$} 
		\end{minipage} 
		\begin{minipage}[b]{0.28\linewidth}
			\centering	{\footnotesize $\sigma=24$} 
		\end{minipage}
		\\
		%---------------------------------------------------
		% true images
		\begin{minipage}[b]{0.1\linewidth}
			\centering
			{\footnotesize Truth}  
		\end{minipage} 
		\begin{minipage}[b]{0.28\linewidth}
			\centering
			\includegraphics[width = 2.5cm, height = 2.5cm]{./Figures/GF/ImgNo8_Noise8_X_true.eps}
		\end{minipage} 
		\begin{minipage}[b]{0.28\linewidth}
			\centering
			\includegraphics[width = 2.5cm, height = 2.5cm]{./Figures/GF/ImgNo8_Noise16_X_true.eps}
		\end{minipage} 
		\begin{minipage}[b]{0.28\linewidth}
			\centering
			\includegraphics[width = 2.5cm, height = 2.5cm]{./Figures/GF/ImgNo8_Noise24_X_true.eps}
		\end{minipage} 
		\\
		% -------------------------------------------
		% JFSM
		\begin{minipage}[b]{0.1\linewidth}
			\centering
			{\footnotesize JFSM\cite{shen2015multispectral}}  
		\end{minipage}  
		\begin{minipage}[b]{0.28\linewidth}
			\centering
			\includegraphics[width = 2.5cm, height = 2.5cm]{./Figures/JFSM/ImgNo8_Noise8_X_JFSM.eps}
		\end{minipage}  
		\begin{minipage}[b]{0.28\linewidth}
			\centering
			\includegraphics[width = 2.5cm, height = 2.5cm]{./Figures/JFSM/ImgNo8_Noise16_X_JFSM.eps}
		\end{minipage} 
		\begin{minipage}[b]{0.28\linewidth}
			\centering
			\includegraphics[width = 2.5cm, height = 2.5cm]{./Figures/JFSM/ImgNo8_Noise24_X_JFSM.eps}
		\end{minipage} 
		\\
		% -------------------------------------------	
		% JFSM
		\begin{minipage}[b]{0.1\linewidth}
			\centering
			{\footnotesize ErrMap JFSM\cite{shen2015multispectral}}  
		\end{minipage} 
		\begin{minipage}[b]{0.28\linewidth}
			\centering
			\includegraphics[width = 2.5cm, height = 2.5cm]{./Figures/JFSM/ImgNo8_Noise8_X_resid_JFSM.eps}
		\end{minipage} 
		\begin{minipage}[b]{0.28\linewidth}
			\centering
			\includegraphics[width = 2.5cm, height = 2.5cm]{./Figures/JFSM/ImgNo8_Noise16_X_resid_JFSM.eps}
		\end{minipage} 
		\begin{minipage}[b]{0.28\linewidth}
			\centering
			\includegraphics[width = 2.5cm, height = 2.5cm]{./Figures/JFSM/ImgNo8_Noise24_X_resid_JFSM.eps}
		\end{minipage} 
		\\
		% -------------------------------------------
		% DJF
		\begin{minipage}[b]{0.1\linewidth}
			\centering
			{\footnotesize DJF~\cite{li2016deep}} %  
		\end{minipage} 
		\begin{minipage}[b]{0.28\linewidth}
			\centering
			\includegraphics[width = 2.5cm, height = 2.5cm]{./Figures/DJF/ImgNo8_Noise8_X_DJF.eps}
		\end{minipage} 
		\begin{minipage}[b]{0.28\linewidth}
			\centering
			\includegraphics[width = 2.5cm, height = 2.5cm]{./Figures/DJF/ImgNo8_Noise16_X_DJF.eps}
		\end{minipage} 
		\begin{minipage}[b]{0.28\linewidth}
			\centering
			\includegraphics[width = 2.5cm, height = 2.5cm]{./Figures/DJF/ImgNo8_Noise24_X_DJF.eps}
		\end{minipage} 
		\\
		% -------------------------------------------
		% DJF
		\begin{minipage}[b]{0.1\linewidth}
			\centering
			{\footnotesize ErrMap DJF~\cite{li2016deep}} %  
		\end{minipage}  
		\begin{minipage}[b]{0.28\linewidth}
			\centering
			\includegraphics[width = 2.5cm, height = 2.5cm]{./Figures/DJF/ImgNo8_Noise8_X_resid_DJF.eps}
		\end{minipage} 
		\begin{minipage}[b]{0.28\linewidth}
			\centering
			\includegraphics[width = 2.5cm, height = 2.5cm]{./Figures/DJF/ImgNo8_Noise16_X_resid_DJF.eps}
		\end{minipage} 
		\begin{minipage}[b]{0.28\linewidth}
			\centering
			\includegraphics[width = 2.5cm, height = 2.5cm]{./Figures/DJF/ImgNo8_Noise24_X_resid_DJF.eps}
		\end{minipage} 
		\\
		% -------------------------------------------
		%	% CDN with standard sparsity
		%	\begin{minipage}[b]{0.1\linewidth}
		%		\centering
		%		{\footnotesize Ours} %  
		%	\end{minipage} 
		%	\begin{minipage}[b]{0.28\linewidth}
		%		\centering
		%		\includegraphics[width = 2.5cm, height = 2.5cm]{./Figures/CDN/ImgNo8_Noise4_X_CDN.eps}
		%	\end{minipage} 
		%	\begin{minipage}[b]{0.28\linewidth}
		%		\centering
		%		\includegraphics[width = 2.5cm, height = 2.5cm]{./Figures/CDN/ImgNo8_Noise12_X_CDN.eps}
		%	\end{minipage} 
		%	\begin{minipage}[b]{0.28\linewidth}
		%		\centering
		%		\includegraphics[width = 2.5cm, height = 2.5cm]{./Figures/CDN/ImgNo8_Noise20_X_CDN.eps}
		%	\end{minipage} 
		%	\\
		% -------------------------------------------
		%	% CDN with standard sparsity
		%	\begin{minipage}[b]{0.1\linewidth}
		%		\centering
		%		{\footnotesize ErrMap Ours} %  
		%	\end{minipage} 
		%	\begin{minipage}[b]{0.28\linewidth}
		%		\centering
		%		\includegraphics[width = 2.5cm, height = 2.5cm]{./Figures/CDN/ImgNo8_Noise8_X_resid_CDN.eps}
		%	\end{minipage} 
		%	\begin{minipage}[b]{0.28\linewidth}
		%		\centering
		%		\includegraphics[width = 2.5cm, height = 2.5cm]{./Figures/CDN/ImgNo8_Noise16_X_resid_CDN.eps}
		%	\end{minipage} 
		%	\begin{minipage}[b]{0.28\linewidth}
		%		\centering
		%		\includegraphics[width = 2.5cm, height = 2.5cm]{./Figures/CDN/ImgNo8_Noise24_X_resid_CDN.eps}
		%	\end{minipage} 
		%	\\
		% -------------------------------------------
		% CDN with group sparsity
		\begin{minipage}[b]{0.1\linewidth}
			\centering
			{\footnotesize Ours+}  
		\end{minipage} 
		\begin{minipage}[b]{0.28\linewidth}
			\centering
			\includegraphics[width = 2.5cm, height = 2.5cm]{./Figures/CDN_GrpSp/ImgNo8_Noise8_X_CDN.eps}
		\end{minipage} 
		\begin{minipage}[b]{0.28\linewidth}
			\centering
			\includegraphics[width = 2.5cm, height = 2.5cm]{./Figures/CDN_GrpSp/ImgNo8_Noise16_X_CDN.eps}
		\end{minipage} 
		\begin{minipage}[b]{0.28\linewidth}
			\centering
			\includegraphics[width = 2.5cm, height = 2.5cm]{./Figures/CDN_GrpSp/ImgNo8_Noise24_X_CDN.eps}
		\end{minipage} 
		\\
		% -------------------------------------------
		% CDN with group sparsity
		\begin{minipage}[b]{0.1\linewidth}
			\centering
			{\footnotesize ErrMap Ours+}  
		\end{minipage} 
		\begin{minipage}[b]{0.28\linewidth}
			\centering
			\includegraphics[width = 2.5cm, height = 2.5cm]{./Figures/CDN_GrpSp/ImgNo8_Noise8_X_resid_CDN.eps}
		\end{minipage} 
		\begin{minipage}[b]{0.28\linewidth}
			\centering
			\includegraphics[width = 2.5cm, height = 2.5cm]{./Figures/CDN_GrpSp/ImgNo8_Noise16_X_resid_CDN.eps}
		\end{minipage} 
		\begin{minipage}[b]{0.28\linewidth}
			\centering
			\includegraphics[width = 2.5cm, height = 2.5cm]{./Figures/CDN_GrpSp/ImgNo8_Noise24_X_resid_CDN.eps}
		\end{minipage} 
		\\
		% ------------------------------------------- 
		\begin{minipage}[b]{0.1\linewidth}
			\centering	% {\phantom{{\footnotesize XXX}}} 
		\end{minipage}
		\begin{minipage}[b]{0.28\linewidth}
			\centering	{\footnotesize $\sigma=8$}
		\end{minipage} 
		\begin{minipage}[b]{0.28\linewidth}
			\centering	{\footnotesize $\sigma=16$} 
		\end{minipage} 
		\begin{minipage}[b]{0.28\linewidth}
			\centering	{\footnotesize $\sigma=24$} 
		\end{minipage}
		% -------------------------------------------	
	\end{multicols}	
	
	\vspace{-0.8cm}
	
	\begin{multicols}{1}  
		\begin{minipage}[b]{0.98\linewidth}
			{\footnotesize Colorbar}
			\includegraphics[width = 16.8cm, height=0.5cm]{./Figures/Colorbar64.eps}
		\end{minipage}
	\end{multicols}	
	
	\vspace{-0.6cm}
	
	\caption{Visual comparison on multimodal image denoising.}
	%	 Each row represents one approach and its denoising results corresponding to different noise levels.}
	\label{Fig:DenoisedIms_8}
\end{figure*}
